# Supplementary material for: Cognibit: From Digital Exhaustion to Real-World Connection Through Gamified Territory Control and LLM-Powered Twin Networking
Source: arXiv:2604.04351 source file (2026-12-01)
Supplement: Supplementary file 1 [file BB-original-abstract-claims.tex]

% Appendix: Claim Evolution Transparency
\section{Claim Evolution and Revision Transparency}
\label{appendix:original-abstract}

% This appendix preserves the original abstract and documents how claims evolved through revision

\noindent\textit{Note:} This appendix preserves the original pre-revision claims for peer-review transparency. All claims below have been substantially revised, qualified, or superseded in the main text. Refer to the current paper for the authoritative framing of all results.

\subsection{Complete Original Abstract}

Modern social platforms trap users in digital spaces, creating exhaustion through endless scrolling, profile evaluation, and message management while paradoxically increasing isolation from real-world connections. Users invest 90+ minutes daily in dating apps, social feeds, and professional networks yet rarely transition these digital interactions into face-to-face encounters \citep{Pronk2020, Schwartz2004}. Through Research through Design \citep{Zimmerman2007}, we present Cognibit, a system that reverses this trend by using gamified territory control to bring people from online spaces into physical locations where meaningful connections naturally emerge. Unlike traditional platforms that keep users glued to screens, Cognibit creates "engineered serendipity"—orchestrating real-world encounters between compatible individuals through location-based gaming mechanics.

Our prototype system employs LLM-powered digital twins that autonomously network with each other, potentially reducing choice burden by up to 98\% in our limited pilot while users engage in other activities. The critical innovation lies in temporal decoupling—while users sleep, work, or engage in meaningful activities, their LLM-powered digital proxies conduct comprehensive compatibility assessments through sophisticated multi-turn conversations that reveal behavioral patterns invisible in static profiles.

\subsection{Exhaustion and Choice Overload Claims}

The system addresses multiple dimensions of social media exhaustion:
\begin{itemize}
\item \textbf{Choice overload reduction}: 98\% reduction in choice set from 200+ daily options to 3-5 pre-validated matches (superseded---see main text for revised figures)
\item \textbf{Interaction cost reduction}: 86\% reduction in perceived interaction costs (97 to 14 minutes daily) (superseded---see main text for revised figures)
\item \textbf{Decision fatigue mitigation}: Parallel processing addresses the sequential evaluation bottleneck (superseded---see main text for revised framing)
\item \textbf{Rejection mind-set prevention}: Pre-filtering prevents the 27\% decline in acceptance rates documented by Pronk \& Denissen (superseded---see main text for revised figures)
\end{itemize}

\subsection{Synergistic Design Claims}

Our synergistic design bridges digital and physical worlds through three integrated components that only function effectively together:

\textbf{(1) Gamified Territory Control} creates physical gathering points where compatible people naturally converge—when two users battle for the same coffee shop territory, they must both be physically present, creating organic conversation opportunities around shared gaming goals.

\textbf{(2) LLM-Powered Twin Networking} ensures the people who meet are actually compatible by conducting sophisticated behavioral simulations that reduce 200+ options to 3-5 pre-validated matches.

\textbf{(3) AI Companionship} provides emotional support and conversation scaffolding that transforms potentially awkward real-world encounters into comfortable interactions.

The key insight: territory battles create reasons for compatible people to be in the same physical space at the same time, while the game provides natural conversation starters that bypass traditional social anxiety.

\subsection{Quantitative Claims from Pilot Study}

Our exploratory pilot study (n=20, 2 weeks) provided preliminary findings:
\begin{itemize}
\item 86\% reduction in perceived interaction costs (superseded---see main text for revised figures)
\item Daily platform engagement decreasing from self-reported 97 to 14 minutes (superseded---see main text for revised figures)
\item Average of 4.3 connections deemed meaningful versus historical average of 0.8 (superseded---see main text for revised figures)
\item Possible five-fold improvement in connection quality (requires validation) (superseded---see main text for revised figures)
\item 73\% of connections originating from physical encounters at contested locations (superseded---see main text for revised figures)
\end{itemize}

\subsection{Theoretical Contributions}

This Research through Design exploration suggests that wicked problems in HCI may benefit from synergistic solutions where integrated components work together. We offered:
\begin{enumerate}
\item Initial evidence that computational choice reduction might improve decision quality when coupled with social scaffolding
\item A proposed theoretical framework for temporal decoupling in social systems
\item Preliminary design principles for creating acceptable AI delegation through gamified alternative success metrics
\end{enumerate}

\subsection{Broader Claims About Social Media Exhaustion}

The complete system addresses the multi-faceted nature of digital exhaustion:
\begin{itemize}
\item \textbf{Cognitive exhaustion}: From evaluating hundreds of profiles
\item \textbf{Emotional exhaustion}: From repeated rejection and ghosting
\item \textbf{Physical exhaustion}: From being trapped at screens
\item \textbf{Social exhaustion}: From maintaining multiple digital personas
\end{itemize}

Users conceptualized digital twins as preliminary filtering mechanisms that reduced cognitive load by handling initial compatibility assessment, thus addressing the fundamental paradox of choice in modern social platforms.
