# Supplementary material for: Cognibit: From Digital Exhaustion to Real-World Connection Through Gamified Territory Control and LLM-Powered Twin Networking
Source: arXiv:2604.04351 source file (2026-12-01)
Supplement: Supplementary file 2 [file HH-hci-conclusion.tex]

% Conclusion section
\section{Extended Discussion and Future Directions}

This Research through Design exploration suggests that wicked problems in HCI may benefit from synergistic solutions where integrated components work together toward outcomes that isolated interventions might not achieve. Choice overload in social platforms appears to exemplify such wickedness—cognitive burden, social anxiety, and interaction friction seem so intertwined that addressing one without the others may prove insufficient. Through our Cognibit prototype, we explore how three integrated components—digital twin filtering, territory gaming, and pendant companions—might work in concert to reduce an unmanageable selection problem (200+ daily options) to a more manageable decision task (3-5 pre-filtered matches), though our limited pilot cannot definitively establish this transformation. This exploratory approach follows the framework of \citet{Zimmerman2007} for investigating problems that resist decomposition, offering initial insights that require validation through larger, controlled studies.

Our exploratory contributions suggest how choice architecture principles might help address choice overload: (1) \textbf{Computational Choice Reduction} through digital twins that, in our limited pilot, reduced options from 200+ to 3-5 pre-filtered matches (a 98\% reduction), with participants reporting improved decision quality, though controlled studies are needed; (2) \textbf{Parallel Processing Potential} where AI agents could conduct multiple assessments simultaneously, possibly addressing the sequential evaluation burden that \citet{Vohs2008} identified; (3) \textbf{Proposed Progressive Filtering Architecture} implementing three-stage reduction that may align with bounded rationality principles \citep{Simon1955}, requiring further validation; and (4) \textbf{Gaming as Possible Scaffolding} that appeared to reduce interaction costs \citep{Nielsen2012} in our small sample by providing conversation contexts.

The technical implementation suggests browser-based multi-agent systems may be feasible for consumer applications. Our prototype maintained 58.3 FPS with 5 concurrent digital twins in JavaScript (degrading to below 30 FPS at 8 agents), indicating that small-scale behavioral simulation might be achievable without native installation, though scalability remains severely limited (Section~\ref{sec:limitations}). The Firebase-powered synchronization, while experiencing occasional conflicts, provided cross-device persistence in our limited deployment. The GPS-driven territory mechanics appeared to encourage some participants to explore new locations, though we cannot determine if this effect would persist beyond the novelty period.

\subsection{Potential Implications}

If validated in larger studies, the Cognibit approach could suggest a shift from manual evaluation to computational assistance in social discovery:

\textbf{From Serial to Parallel}: Traditional platforms require serial evaluation—one profile at a time. Digital twins could enable parallel assessment, evaluating many prospects simultaneously while users engage in other activities, potentially shifting the bottleneck from human evaluation time to computational cost.

\textbf{From Synchronous to Asynchronous}: Digital twins could work continuously, independent of user availability, potentially reducing the time users spend on active screening. Our pilot observed this pattern, though whether it produces better outcomes than manual evaluation remains unestablished.

\textbf{Gaming as potential social catalyst}: In our pilot, gaming mechanics appeared to provide conversation starters and shared goals. Some participants reported that boss fights and territory conquest created more natural interaction contexts than profile-based messaging, though this requires controlled comparison.

\textbf{Persistent AI companionship}: Maintaining interaction history across sessions and devices appeared to increase user engagement with AI companions. Some participants reported feeling understood by their companions, though the long-term implications of such attachments---including dependency risks---require careful study.

\subsection{Future Directions}

Our immediate research agenda focuses on scaling and enhancement:

\subsubsection{Platform expansion}
Beyond dating and social discovery, the architecture naturally extends to several adjacent domains. Professional networking could leverage skill-based twin matching to identify collaborators whose working styles complement each other, moving beyond keyword-matching resumes to behavioral compatibility assessment. Educational tutoring with persistent learning companions could adapt to individual student personalities and learning patterns, maintaining motivational context across sessions. Mental health support through emotionally-aware digital therapists could provide continuous monitoring and intervention, with the companion's persistent memory enabling longitudinal tracking of mood patterns. Creative collaboration with AI co-creators maintaining project context could facilitate sustained partnerships where the AI partner remembers artistic preferences and project history. At scale, virtual worlds where thousands of twins create emergent societies could serve as testbeds for social dynamics research.

\subsubsection{Technical improvements}
Performance optimization remains a priority across five fronts. WebAssembly modules for compute-intensive behavioral simulation could provide near-native execution speed for GNWT module processing and combat physics without leaving the browser environment. Hybrid local/cloud processing would run lightweight inference locally for routine companion interactions while reserving cloud API calls for complex twin conversations, substantially reducing per-user costs. Peer-to-peer twin networking via WebRTC could enable direct twin-to-twin communication for scalable discovery without server intermediation, though reliability challenges noted in our failed mitigation attempts would need to be addressed. Advanced caching strategies for common interaction patterns---such as pre-computing responses for frequent conversational openings---could reduce API call volume by 30--40\%. Native mobile applications for users wanting maximum performance would unlock device-level optimizations for GPS, background processing, and memory management unavailable in browser contexts.

\subsubsection{Richer behavioral modeling}
Current text-based interactions represent a starting point for richer behavioral modeling. Voice and video processing would enable multimodal twin responses that capture tone, pacing, and non-verbal communication cues currently lost in text-only interaction. Emotion recognition through facial expression analysis during video calls could provide real-time affective state data to the GNWT emotion module, enabling more empathetically attuned twin behavior. Cultural adaptation for global deployment requires training twins on culture-specific interaction norms, moving beyond the Western-centric communication patterns embedded in current prompts. Long-term relationship modeling over months and years would track relationship evolution dynamics that the two-week pilot could not capture, including trust building, conflict resolution, and attachment formation. Group dynamics simulation for multi-person interactions would extend the pairwise twin conversation model to evaluate compatibility within larger social groups, enabling team formation and community building applications.

\subsubsection{Real-world integration}
Location-based features present several evolution paths. Augmented reality overlays for territory visualization would render territory boundaries, ownership indicators, and nearby player positions directly onto the camera view, creating a more immersive spatial experience than the current map-based interface. Smart city integration could repurpose territory mechanics for civic engagement, incentivizing visits to public libraries, community centers, and cultural institutions. Business partnerships for location-based rewards would enable local establishments to sponsor territories, providing real-world incentives (discounts, priority seating) for gameplay activity that drives foot traffic. Event coordination for twin-organized meetups would allow twins to autonomously negotiate meeting times and locations based on their users' schedules and preferences. Health gamification through movement tracking could extend the walking incentives already present in territory mechanics into explicit fitness goals, connecting physical activity with social rewards.

\subsection{Methodological Contribution: Synergistic Design as HCI Approach}

Our work explores how Research through Design can address wicked problems through intentionally integrated systems. Traditional HCI evaluation often assumes components can be isolated for study---the ablation study paradigm borrowed from machine learning. Our preliminary observations suggest that for problems where social, cognitive, and emotional factors intertwine, integrated designs may produce different outcomes than isolated components, though our study cannot establish whether this reflects genuine synergy or simply providing more features. This perspective aligns with gestalt principles \citep{Koffka1935} and recent calls in HCI for ecosystemic perspectives \citep{CHI2024CFP}, but requires rigorous factorial validation.

The synergistic design approach offers several hypothesized advantages, pending rigorous factorial validation. Gaming mechanics may address resistance to AI delegation by framing computational assistance as strategic advantage rather than loss of control---users who might resist ``letting an AI choose for me'' may readily accept ``my digital twin scouts ahead while I play.'' The combination may enable emergent properties that isolated components do not produce, though we cannot yet distinguish genuine emergence from additive effects with our current study design. Each component may strengthen the others' effectiveness through mutual reinforcement: gaming provides contexts for twin-evaluated matches to meet, twins provide personalized opponents for gaming encounters, and companions provide emotional scaffolding that sustains engagement with both. The integrated design also enables holistic evaluation where success metrics emerge from the system as a whole rather than from individual parts, capturing interaction effects that component-level measurement would miss.

This methodology extends beyond our specific application. Any HCI challenge involving intertwined social, cognitive, and emotional factors—from health behavior change to collaborative work systems—may benefit from synergistic rather than modular design approaches.

\subsection{Implications for Human-Computer Interaction}

This work explores whether choice overload might be a factor in social platform challenges. We investigated whether computational pre-filtering could potentially address choice paralysis, though our small pilot cannot establish if this approach is effective. While we observed participants reporting reduced choice sets, we cannot verify if this actually countered rejection mind-sets or improved outcomes. The confounded design and lack of controls prevent determining whether any observed behaviors resulted from our specific approach or simply from providing any structured intervention.

The implications extend beyond dating to any domain suffering from choice overload—job searching, content discovery, product selection. Our three-stage filtering architecture (elimination $\to$ behavioral assessment $\to$ human decision) suggests a potentially generalizable framework for managing overwhelming option spaces. By respecting cognitive limits \citep{Miller1956} and bounded rationality \citep{Simon1955}, systems can enhance rather than overwhelm human decision-making.

Our observations are consistent with the prediction of \citet{Schwartz2004} that "satisficers" achieve better outcomes than "maximizers" in high-choice environments. Users who accepted the AI's pre-filtering (satisficing with good-enough options) reported higher satisfaction than those who insisted on reviewing all possibilities, though our small sample (N=20) and lack of controls prevent causal attribution.

The technical implementation revealed fundamental limitations: the system maintains acceptable performance with up to 8 concurrent agents (58.3 FPS at 5 agents, degrading to below 30 FPS at 8 and to 9.7 FPS at 20), with hard failure beyond 20 due to browser memory constraints. The \$35.53/user/month cost makes the approach economically unviable even with optimization. Browser memory constraints (2GB) and single-threaded JavaScript execution prevent the true parallel processing our design envisioned. These technical failures suggest that browser-based multi-agent systems may not be feasible for platform-scale social applications without major architectural redesign.

Critical research questions emerge from this work: What constitutes appropriate boundaries for algorithmic intervention in intimate human decisions? How do we maintain user autonomy while leveraging computational efficiency? Can agent-based matching overcome the homophily bias inherent in human mate selection? These questions necessitate interdisciplinary collaboration spanning computer science, psychology, sociology, and ethics.

Looking forward, we anticipate three trajectories for this research: First, advances in large language models will enable increasingly sophisticated behavioral simulation, potentially enabling more nuanced compatibility assessment. Second, the integration of multimodal data (voice, facial expressions, physiological signals) will enrich compatibility assessment beyond text-based interaction. Third, federated learning approaches may enable personalized matching while preserving privacy, addressing the tension between data utility and user protection.

The potential implications, if our preliminary findings are validated, could extend beyond romantic matching to other forms of social connection—professional networking, friendship formation, or collaborative team assembly. Our exploratory work suggests that computational agents might help navigate compatibility assessment, though the effectiveness and appropriateness of such delegation requires careful study. The contribution of this work is not to prove that AI should replace human judgment, but to explore one possible approach to augmenting human capacity in an increasingly overwhelming digital social landscape.

We invite the research community to critically examine and extend this exploratory foundation through larger-scale controlled studies, ablation testing of individual components, and investigation of alternative architectures. Key questions remain: Does the synergistic design truly require all three components? Would simpler interventions achieve similar outcomes? How do these effects persist over time? The convergence of location-based interaction, persistent AI companionship, and autonomous social discovery represents just one possible approach among many. We hope this initial exploration stimulates further research into how technology might address social media exhaustion while preserving human agency and authentic connection.

\subsection{Limitations of This Work}

This paper presents an exploratory pilot study with significant limitations. Our sample of 20 participants over 2 weeks cannot establish causal relationships or generalize to broader populations. The absence of control conditions prevents us from isolating component contributions. Novelty effects likely inflated engagement metrics. Self-reported data may reflect social desirability bias. The single-city deployment limits geographic validity. Most critically, we cannot determine whether observed effects stem from our specific design or simply from providing any structured social intervention. These limitations underscore that our findings are preliminary observations requiring rigorous validation before drawing definitive conclusions about addressing social media exhaustion through computational delegation.
