# Supplementary material for: Cognibit: From Digital Exhaustion to Real-World Connection Through Gamified Territory Control and LLM-Powered Twin Networking
Source: arXiv:2604.04351 source file (2026-12-01)
Supplement: Supplementary file 3 [file O-ai-behavior-tree.tex]

% Appendix O - AI Behavior Tree Architecture
\section{AI Behavior Tree Architecture}

This appendix presents the hierarchical behavior tree system used for complex AI decision-making, particularly for boss encounters and advanced NPC behaviors.

\subsection{Behavior Tree Node Types}

The behavior tree implements three fundamental node types:
\begin{itemize}
\item \textbf{Selector}: Tries children until one succeeds (OR logic)
\item \textbf{Sequence}: Requires all children to succeed (AND logic)
\item \textbf{Action}: Leaf nodes that execute specific behaviors
\end{itemize}

\begin{algorithm}[!htbp]
\caption{Behavior Tree Node Execution}
\label{alg:behavior-tree-execution}
\begin{algorithmic}[1]
\Require Node structure, Game state, Delta time
\Ensure Action selection or failure status

\State \textbf{Node Types:}
\State SELECTOR, SEQUENCE, ACTION
\State \textbf{Return Status:}
\State SUCCESS, FAILURE, RUNNING

\Function{ExecuteBehaviorNode}{node, gameState, deltaTime}
    \State \Comment{Route to appropriate node handler}
    \If{node.type = SELECTOR}
        \State \Return \Call{ExecuteSelector}{node, gameState, deltaTime}
    \ElsIf{node.type = SEQUENCE}
        \State \Return \Call{ExecuteSequence}{node, gameState, deltaTime}
    \ElsIf{node.type = ACTION}
        \State \Return \Call{ExecuteAction}{node, gameState, deltaTime}
    \Else
        \State \Return \{status: FAILURE\}
    \EndIf
\EndFunction

\Function{ExecuteSelector}{node, gameState, deltaTime}
    \State \Comment{Try each child until one succeeds}
    \ForAll{child $\in$ node.children}
        \If{child.condition $\neq$ null}
            \If{\textbf{not} \Call{EvaluateCondition}{child.condition, gameState}}
                \State \textbf{continue} \Comment{Skip if condition fails}
            \EndIf
        \EndIf

        \State result $\gets$ \Call{ExecuteBehaviorNode}{child, gameState, deltaTime}

        \If{result.status = SUCCESS \textbf{or} result.status = RUNNING}
            \State \Return result
        \EndIf
    \EndFor

    \State \Return \{status: FAILURE\}
\EndFunction

\Function{ExecuteSequence}{node, gameState, deltaTime}
    \State \Comment{All children must succeed}
    \If{node.condition $\neq$ null}
        \If{\textbf{not} \Call{EvaluateCondition}{node.condition, gameState}}
            \State \Return \{status: FAILURE\}
        \EndIf
    \EndIf

    \ForAll{child $\in$ node.children}
        \State result $\gets$ \Call{ExecuteBehaviorNode}{child, gameState, deltaTime}

        \If{result.status = FAILURE}
            \State \Return \{status: FAILURE\}
        \ElsIf{result.status = RUNNING}
            \State \Return \{status: RUNNING\}
        \EndIf
    \EndFor

    \State \Return \{status: SUCCESS\}
\EndFunction

\Function{ExecuteAction}{node, gameState, deltaTime}
    \State \Comment{Execute leaf node action}
    \State \Return \{
    \State \quad status: SUCCESS,
    \State \quad action: node.action,
    \State \quad damage: node.damage || 50,
    \State \quad effects: node.effects || [],
    \State \quad animation: node.animation || node.action
    \State \}
\EndFunction

\end{algorithmic}
\end{algorithm}

\subsection{Boss AI Decision Making}

The boss AI system uses behavior trees with condition-based branching to create adaptive and challenging combat encounters.

\begin{algorithm}[!htbp]
\caption{Dragon Boss AI Behavior Tree}
\label{alg:dragon-boss-ai}
\begin{algorithmic}[1]
\Require Boss state, Player state, Battle context, Difficulty $d \in [0.5, 2.0]$
\Ensure Selected action with damage and effects

\State \textbf{Blackboard Variables:}
\State healthPercent $\gets$ boss.health / boss.maxHealth
\State playerDistance $\gets$ \Call{CalculateDistance}{boss.position, player.position}
\State battleDuration $\gets$ currentTime - battle.startTime
\State teamSize $\gets$ battle.teamSize || 1

\Function{CreateDragonBehaviorTree}{difficulty}
    \State \Return \{
    \State \quad type: SELECTOR,
    \State \quad children: [
    \State \quad \quad \Call{CreateCriticalPhase}{difficulty},
    \State \quad \quad \Call{CreateRangedPhase}{difficulty},
    \State \quad \quad \Call{CreateMeleePhase}{difficulty}
    \State \quad ]
    \State \}
\EndFunction

\Function{CreateCriticalPhase}{difficulty}
    \State \Comment{Low health emergency behaviors}
    \State \Return \{
    \State \quad type: SEQUENCE,
    \State \quad condition: healthPercent $< 0.3$,
    \State \quad children: [
    \State \quad \quad \{type: ACTION, action: 'retreat\_and\_heal', priority: 1\},
    \State \quad \quad \{type: ACTION, action: 'summon\_minions', priority: 2\},
    \State \quad \quad \{type: ACTION, action: 'berserker\_rage', priority: 3\}
    \State \quad ]
    \State \}
\EndFunction

\Function{CreateRangedPhase}{difficulty}
    \State \Comment{Long-distance attack patterns}
    \State \Return \{
    \State \quad type: SEQUENCE,
    \State \quad condition: playerDistance $> 20$,
    \State \quad children: [
    \State \quad \quad \{type: ACTION, action: 'aerial\_dive', damage: $150 \times difficulty$\},
    \State \quad \quad \{type: ACTION, action: 'fire\_barrage', damage: $120 \times difficulty$\},
    \State \quad \quad \{type: ACTION, action: 'wing\_gust', damage: $80 \times difficulty$\}
    \State \quad ]
    \State \}
\EndFunction

\Function{CreateMeleePhase}{difficulty}
    \State \Comment{Close-combat attack patterns}
    \State \Return \{
    \State \quad type: SEQUENCE,
    \State \quad condition: playerDistance $\leq 20$,
    \State \quad children: [
    \State \quad \quad \{type: ACTION, action: 'claw\_combo', damage: $100 \times difficulty$\},
    \State \quad \quad \{type: ACTION, action: 'tail\_whip', damage: $90 \times difficulty$\},
    \State \quad \quad \{type: ACTION, action: 'ground\_breath', damage: $110 \times difficulty$\}
    \State \quad ]
    \State \}
\EndFunction

\end{algorithmic}
\end{algorithm}

\subsection{Adaptive Difficulty System}

The AI adapts its behavior based on player performance and team composition, creating dynamic challenge scaling.

\begin{algorithm}[!htbp]
\caption{Adaptive AI Difficulty Adjustment}
\label{alg:adaptive-difficulty}
\begin{algorithmic}[1]
\Require Player metrics, Team composition, Battle history
\Ensure Adjusted difficulty multiplier $d \in [0.5, 2.0]$

\State \textbf{Initialize:}
\State baseDifficulty $\gets 1.0$
\State adaptationRate $\gets 0.1$
\State performanceWindow $\gets 300$ seconds

\Function{CalculateAdaptiveDifficulty}{playerMetrics, battleHistory}
    \State \Comment{Analyze recent player performance}
    \State recentBattles $\gets$ \Call{GetRecentBattles}{battleHistory, performanceWindow}
    \State winRate $\gets$ \Call{CalculateWinRate}{recentBattles}
    \State avgTimeToVictory $\gets$ \Call{AverageVictoryTime}{recentBattles}
    \State deathCount $\gets$ \Call{CountPlayerDeaths}{recentBattles}

    \State \Comment{Calculate performance score}
    \State performanceScore $\gets 0.5$
    \State performanceScore $\gets$ performanceScore $+ (winRate - 0.5) \times 0.3$
    \State performanceScore $\gets$ performanceScore $- (deathCount / 10) \times 0.2$

    \If{avgTimeToVictory $< 60$} \Comment{Quick victories}
        \State performanceScore $\gets$ performanceScore $+ 0.2$
    \ElsIf{avgTimeToVictory $> 300$} \Comment{Struggling}
        \State performanceScore $\gets$ performanceScore $- 0.2$
    \EndIf

    \State \Comment{Apply team size modifier}
    \State teamModifier $\gets 1.0 + (playerMetrics.teamSize - 1) \times 0.15$

    \State \Comment{Calculate final difficulty}
    \State targetDifficulty $\gets$ baseDifficulty

    \If{performanceScore $> 0.7$}
        \State targetDifficulty $\gets$ targetDifficulty $+ adaptationRate$
    \ElsIf{performanceScore $< 0.3$}
        \State targetDifficulty $\gets$ targetDifficulty $- adaptationRate$
    \EndIf

    \State targetDifficulty $\gets$ targetDifficulty $\times$ teamModifier
    \State targetDifficulty $\gets$ \Call{Clamp}{targetDifficulty, 0.5, 2.0}

    \State \Comment{Smooth difficulty transitions}
    \State currentDifficulty $\gets$ playerMetrics.currentDifficulty || baseDifficulty
    \State smoothedDifficulty $\gets$ currentDifficulty $\times 0.8 + targetDifficulty \times 0.2$

    \State \Return smoothedDifficulty
\EndFunction

\Function{ApplyDifficultyToAI}{aiTree, difficulty}
    \State \Comment{Scale AI parameters}
    \ForAll{action $\in$ \Call{GetAllActions}{aiTree}}
        \State action.damage $\gets$ action.baseDamage $\times$ difficulty
        \State action.cooldown $\gets$ action.baseCooldown / difficulty
        \State action.accuracy $\gets$ \Call{Min}{1.0, action.baseAccuracy $\times$ difficulty}
    \EndFor

    \State \Comment{Adjust decision thresholds}
    \ForAll{condition $\in$ \Call{GetAllConditions}{aiTree}}
        \If{condition.type = 'health\_threshold'}
            \State condition.threshold $\gets$ condition.baseThreshold $\times$ (2 - difficulty)
        \EndIf
    \EndFor

    \State \Return aiTree
\EndFunction

\end{algorithmic}
\end{algorithm}

\subsection{Multi-Agent Coordination}

For encounters with multiple AI-controlled entities, the system implements coordination protocols to create tactical group behaviors.

\begin{algorithm}[!htbp]
\caption{Multi-Agent AI Coordination}
\label{alg:multi-agent-coordination}
\begin{algorithmic}[1]
\Require Agent list, Shared blackboard, Target priorities
\Ensure Coordinated action plan for all agents

\State \textbf{Coordination Roles:}
\State LEADER, SUPPORT, FLANKER, RANGED

\Function{CoordinateMultiAgentBehavior}{agents, sharedBlackboard}
    \State \Comment{Elect tactical leader}
    \State leader $\gets$ \Call{SelectLeader}{agents}
    \State \Call{AssignRoles}{agents, leader}

    \State \Comment{Share tactical information}
    \ForAll{agent $\in$ agents}
        \State \Call{UpdateSharedKnowledge}{agent, sharedBlackboard}
    \EndFor

    \State \Comment{Coordinate attack patterns}
    \State tacticalPlan $\gets$ \Call{CreateTacticalPlan}{leader, agents}

    \ForAll{agent $\in$ agents}
        \State agentPlan $\gets$ \Call{GetRolePlan}{tacticalPlan, agent.role}
        \State agent.currentPlan $\gets$ agentPlan
        \State \Call{ExecutePlan}{agent, agentPlan}
    \EndFor
\EndFunction

\Function{SelectLeader}{agents}
    \State \Comment{Choose most suitable leader}
    \State bestScore $\gets -\infty$
    \State leader $\gets$ null

    \ForAll{agent $\in$ agents}
        \State score $\gets 0$
        \State score $\gets$ score $+ agent.health / agent.maxHealth \times 0.3$
        \State score $\gets$ score $+ agent.level \times 0.2$
        \State score $\gets$ score $+ agent.intelligence \times 0.3$
        \State score $\gets$ score $+ agent.aliveTime \times 0.2$

        \If{score $> bestScore$}
            \State bestScore $\gets$ score
            \State leader $\gets$ agent
        \EndIf
    \EndFor

    \State \Return leader
\EndFunction

\Function{CreateTacticalPlan}{leader, agents}
    \State playerPositions $\gets$ \Call{GetPlayerPositions}{}
    \State threatLevel $\gets$ \Call{AssessThreat}{playerPositions}

    \State plan $\gets$ \{
    \State \quad formation: null,
    \State \quad primaryTarget: null,
    \State \quad tactics: []
    \State \}

    \If{threatLevel $> 0.7$}
        \State plan.formation $\gets$ 'defensive\_circle'
        \State plan.tactics $\gets$ ['focus\_fire', 'retreat\_wounded']
    \ElsIf{\Call{Size}{agents} $> 3$}
        \State plan.formation $\gets$ 'pincer\_movement'
        \State plan.tactics $\gets$ ['flanking', 'crossfire']
    \Else
        \State plan.formation $\gets$ 'aggressive\_rush'
        \State plan.tactics $\gets$ ['overwhelm', 'chain\_combos']
    \EndIf

    \State plan.primaryTarget $\gets$ \Call{SelectPrimaryTarget}{playerPositions}

    \State \Return plan
\EndFunction

\end{algorithmic}
\end{algorithm}
