# Supplementary material for: Cognibit: From Digital Exhaustion to Real-World Connection Through Gamified Territory Control and LLM-Powered Twin Networking
Source: arXiv:2604.04351 source file (2026-12-01)
Supplement: Supplementary file 4 [file P-procedural-generation.tex]

% Appendix P - Procedural Generation Systems
\section{Procedural Generation Systems}

This appendix details the procedural generation algorithms used for creating unique, explorable environments including castles, dungeons, and world features.

\subsection{Castle Generation Pipeline}

The procedural castle generation system creates unique architectural structures based on templates, biome parameters, and size configurations.

\begin{algorithm}[!htbp]
\caption{Procedural Castle Generation}
\label{alg:procedural-castle-generation}
\begin{algorithmic}[1]
\Require Castle type, Size, Biome
\Ensure Complete castle structure with interactive elements

\State \textbf{Castle Types:}
\State classic, fortress, mystical, dark
\State \textbf{Size Categories:}
\State small (0.7x), medium (1.0x), large (1.4x), massive (2.0x)
\State \textbf{Biome Types:}
\State temperate, desert, arctic, volcanic, forest

\Function{GenerateProceduralCastle}{castleType, size, biome}
    \State \Comment{Initialize generation parameters}
    \State template $\gets$ \Call{GetCastleTemplate}{castleType}
    \State config $\gets$ \Call{GenerateConfig}{size, biome}
    \State seed $\gets$ \Call{Random}{} $\times 10000$

    \State \Comment{Generate main structures}
    \State keep $\gets$ \Call{GenerateKeep}{template, config}
    \State towers $\gets$ \Call{GenerateTowers}{template, config}
    \State walls $\gets$ \Call{GenerateWalls}{template, config}
    \State door $\gets$ \Call{GenerateCastleDoor}{config}

    \State \Comment{Apply biome-specific modifications}
    \State \Call{ApplyBiomeStyle}{keep, towers, walls, biome}

    \State \Comment{Add unique features}
    \State features $\gets$ \Call{GenerateUniqueFeatures}{castleType, config}
    \ForAll{feature $\in$ features}
        \State \Call{PlaceFeature}{feature, keep}
    \EndFor

    \State \Comment{Generate metadata}
    \State lore $\gets$ \Call{GenerateCastleLore}{castleType, biome}
    \State castleId $\gets$ "procedural\_castle\_" + \Call{Floor}{seed}

    \State \Return \{
    \State \quad structure: \{keep, towers, walls, door\},
    \State \quad config: config,
    \State \quad lore: lore,
    \State \quad uniqueFeatures: features,
    \State \quad id: castleId
    \State \}
\EndFunction

\Function{GetCastleTemplate}{castleType}
    \State templates $\gets$ \{
    \State \quad classic: \{
    \State \quad \quad style: 'medieval',
    \State \quad \quad towers: \{min: 4, max: 8\},
    \State \quad \quad walls: \{height: 15, thickness: 3\},
    \State \quad \quad features: ['great\_hall', 'throne\_room', 'armory']
    \State \quad \},
    \State \quad fortress: \{
    \State \quad \quad style: 'military',
    \State \quad \quad towers: \{min: 6, max: 12\},
    \State \quad \quad walls: \{height: 20, thickness: 5\},
    \State \quad \quad features: ['barracks', 'war\_room', 'weapon\_forge']
    \State \quad \},
    \State \quad mystical: \{
    \State \quad \quad style: 'magical',
    \State \quad \quad towers: \{min: 3, max: 6\},
    \State \quad \quad walls: \{height: 25, thickness: 2\},
    \State \quad \quad features: ['spell\_library', 'alchemy\_lab', 'portal\_room']
    \State \quad \},
    \State \quad dark: \{
    \State \quad \quad style: 'gothic',
    \State \quad \quad towers: \{min: 5, max: 10\},
    \State \quad \quad walls: \{height: 18, thickness: 4\},
    \State \quad \quad features: ['dark\_throne', 'torture\_chamber', 'shadow\_vault']
    \State \quad \}
    \State \}

    \State \Return templates[castleType] || templates.classic
\EndFunction

\end{algorithmic}
\end{algorithm}

\subsection{Tower and Wall Generation}

The system procedurally places towers and walls based on mathematical patterns and template constraints.

\begin{algorithm}[!htbp]
\caption{Tower and Wall Placement}
\label{alg:tower-wall-generation}
\begin{algorithmic}[1]
\Require Template, Configuration, Random seed
\Ensure Positioned tower and wall elements

\Function{GenerateTowers}{template, config}
    \State towers $\gets []$
    \State towerCount $\gets$ \Call{RandomInt}{template.towers.min, template.towers.max}
    \State radius $\gets 40 \times$ config.sizeMultiplier

    \ForAll{i $\in [0, towerCount)$}
        \State angle $\gets (i / towerCount) \times 2\pi$
        \State x $\gets$ \Call{Cos}{angle} $\times$ radius
        \State z $\gets$ \Call{Sin}{angle} $\times$ radius

        \State \Comment{Vary tower dimensions}
        \State height $\gets (20 + \Call{Random}{} \times 15) \times$ config.sizeMultiplier
        \State towerRadius $\gets (3 + \Call{Random}{} \times 2) \times$ config.sizeMultiplier

        \State tower $\gets$ \{
        \State \quad position: \{x: x, y: height/2, z: z\},
        \State \quad height: height,
        \State \quad radius: towerRadius,
        \State \quad type: \Call{SelectTowerType}{template.style}
        \State \}

        \State \Comment{Add architectural details}
        \State \Call{AddTowerRoof}{tower, config}
        \State \Call{AddTowerWindows}{tower, height}

        \If{template.style = 'mystical'}
            \State \Call{AddMagicalAura}{tower}
        \EndIf

        \State \Call{Add}{towers, tower}
    \EndFor

    \State \Return towers
\EndFunction

\Function{GenerateWalls}{template, config}
    \State walls $\gets []$
    \State wallSegments $\gets 8$
    \State radius $\gets 35 \times$ config.sizeMultiplier
    \State wallHeight $\gets$ template.walls.height $\times$ config.sizeMultiplier
    \State wallThickness $\gets$ template.walls.thickness

    \ForAll{i $\in [0, wallSegments)$}
        \State angle1 $\gets (i / wallSegments) \times 2\pi$
        \State angle2 $\gets ((i + 1) / wallSegments) \times 2\pi$

        \State x1 $\gets$ \Call{Cos}{angle1} $\times$ radius
        \State z1 $\gets$ \Call{Sin}{angle1} $\times$ radius
        \State x2 $\gets$ \Call{Cos}{angle2} $\times$ radius
        \State z2 $\gets$ \Call{Sin}{angle2} $\times$ radius

        \State wallLength $\gets$ \Call{Sqrt}{$(x2 - x1)^2 + (z2 - z1)^2$}

        \State wall $\gets$ \{
        \State \quad position: \{x: (x1 + x2)/2, y: wallHeight/2, z: (z1 + z2)/2\},
        \State \quad rotation: \Call{Atan2}{z2 - z1, x2 - x1},
        \State \quad length: wallLength,
        \State \quad height: wallHeight,
        \State \quad thickness: wallThickness
        \State \}

        \State \Comment{Add wall features}
        \If{i \% 2 = 0}
            \State \Call{AddBattlements}{wall}
        \EndIf

        \State \Call{Add}{walls, wall}
    \EndFor

    \State \Return walls
\EndFunction

\end{algorithmic}
\end{algorithm}

\subsection{Biome-Specific Styling}

The generation system applies biome-specific materials, colors, and architectural features to create environmental coherence.

\begin{algorithm}[!htbp]
\caption{Biome-Based Style Application}
\label{alg:biome-styling}
\begin{algorithmic}[1]
\Require Structure elements, Biome type
\Ensure Biome-styled architecture

\Function{ApplyBiomeStyle}{structures, biome}
    \State biomeModifiers $\gets$ \Call{GetBiomeModifiers}{biome}

    \ForAll{structure $\in$ structures}
        \State \Comment{Apply material properties}
        \State structure.material $\gets$ biomeModifiers.material
        \State structure.color $\gets$ biomeModifiers.color
        \State structure.roughness $\gets$ biomeModifiers.roughness
        \State structure.metalness $\gets$ biomeModifiers.metalness

        \State \Comment{Apply environmental effects}
        \If{biome = 'desert'}
            \State \Call{ApplySandErosion}{structure}
            \State \Call{AddSandDrifts}{structure}
        \ElsIf{biome = 'arctic'}
            \State \Call{ApplyFrostEffect}{structure}
            \State \Call{AddIcicles}{structure}
        \ElsIf{biome = 'forest'}
            \State \Call{ApplyMossGrowth}{structure}
            \State \Call{AddVines}{structure}
        \ElsIf{biome = 'volcanic'}
            \State \Call{ApplyScorchMarks}{structure}
            \State \Call{AddLavaVeins}{structure}
        \EndIf
    \EndFor
\EndFunction

\Function{GetBiomeModifiers}{biome}
    \State modifiers $\gets$ \{
    \State \quad temperate: \{
    \State \quad \quad material: 'stone',
    \State \quad \quad color: 0x8a7968,
    \State \quad \quad roughness: 0.9,
    \State \quad \quad metalness: 0.05
    \State \quad \},
    \State \quad desert: \{
    \State \quad \quad material: 'sandstone',
    \State \quad \quad color: 0xddbf94,
    \State \quad \quad roughness: 0.95,
    \State \quad \quad metalness: 0.02
    \State \quad \},
    \State \quad arctic: \{
    \State \quad \quad material: 'ice\_stone',
    \State \quad \quad color: 0xb8c5d1,
    \State \quad \quad roughness: 0.3,
    \State \quad \quad metalness: 0.1
    \State \quad \},
    \State \quad volcanic: \{
    \State \quad \quad material: 'obsidian',
    \State \quad \quad color: 0x2c1810,
    \State \quad \quad roughness: 0.2,
    \State \quad \quad metalness: 0.4
    \State \quad \},
    \State \quad forest: \{
    \State \quad \quad material: 'moss\_stone',
    \State \quad \quad color: 0x6b7c5a,
    \State \quad \quad roughness: 0.85,
    \State \quad \quad metalness: 0.05
    \State \quad \}
    \State \}

    \State \Return modifiers[biome] || modifiers.temperate
\EndFunction

\end{algorithmic}
\end{algorithm}

\subsection{Interior Room Generation}

The system generates interconnected interior rooms with proper navigation paths and feature placement.

\begin{algorithm}[!htbp]
\caption{Interior Room Layout Generation}
\label{alg:room-generation}
\begin{algorithmic}[1]
\Require Castle template, Available space, Feature list
\Ensure Connected room graph with placed features

\State \textbf{Room Types:}
\State entrance, corridor, chamber, hall, special
\State \textbf{Connection Types:}
\State door, archway, staircase, secret\_passage

\Function{GenerateInteriorLayout}{template, keepDimensions}
    \State rooms $\gets []$
    \State connections $\gets []$
    \State grid $\gets$ \Call{CreateGrid}{keepDimensions.width, keepDimensions.depth}

    \State \Comment{Place mandatory entrance}
    \State entrance $\gets$ \Call{PlaceRoom}{grid, 'entrance', \{x: 0, z: 0\}}
    \State \Call{Add}{rooms, entrance}

    \State \Comment{Generate room placement}
    \ForAll{feature $\in$ template.features}
        \State roomType $\gets$ \Call{GetRoomTypeForFeature}{feature}
        \State position $\gets$ \Call{FindValidPosition}{grid, roomType}

        \If{position $\neq$ null}
            \State room $\gets$ \Call{PlaceRoom}{grid, roomType, position}
            \State room.feature $\gets$ feature
            \State \Call{Add}{rooms, room}
        \EndIf
    \EndFor

    \State \Comment{Ensure connectivity}
    \State \Call{ConnectRooms}{rooms, connections}

    \State \Comment{Add corridors where needed}
    \State corridors $\gets$ \Call{GenerateCorridors}{rooms, grid}
    \State rooms $\gets$ rooms $\cup$ corridors

    \State \Return \{
    \State \quad rooms: rooms,
    \State \quad connections: connections,
    \State \quad navigationGraph: \Call{BuildNavigationGraph}{rooms, connections}
    \State \}
\EndFunction

\Function{ConnectRooms}{rooms, connections}
    \State \Comment{Create minimum spanning tree}
    \State mst $\gets$ \Call{CreateMST}{rooms}

    \ForAll{edge $\in$ mst}
        \State room1 $\gets$ edge.source
        \State room2 $\gets$ edge.target

        \State connectionType $\gets$ \Call{SelectConnectionType}{room1, room2}
        \State connection $\gets$ \{
        \State \quad from: room1.id,
        \State \quad to: room2.id,
        \State \quad type: connectionType,
        \State \quad position: \Call{CalculateDoorPosition}{room1, room2}
        \State \}

        \State \Call{Add}{connections, connection}
    \EndFor

    \State \Comment{Add additional connections for cycles}
    \State cycleCount $\gets$ \Call{Floor}{\Call{Size}{rooms} $\times 0.3$}
    \ForAll{i $\in [0, cycleCount)$}
        \State room1 $\gets$ \Call{RandomChoice}{rooms}
        \State room2 $\gets$ \Call{FindNearbyRoom}{room1, rooms}

        \If{\textbf{not} \Call{AreConnected}{room1, room2, connections}}
            \State connection $\gets$ \Call{CreateConnection}{room1, room2, 'secret\_passage'}
            \State \Call{Add}{connections, connection}
        \EndIf
    \EndFor
\EndFunction

\Function{PlaceRoom}{grid, roomType, position}
    \State roomSizes $\gets$ \{
    \State \quad entrance: \{width: 3, height: 3\},
    \State \quad corridor: \{width: 2, height: 5\},
    \State \quad chamber: \{width: 4, height: 4\},
    \State \quad hall: \{width: 6, height: 8\},
    \State \quad special: \{width: 5, height: 5\}
    \State \}

    \State size $\gets$ roomSizes[roomType]
    \State room $\gets$ \{
    \State \quad id: \Call{GenerateId}{},
    \State \quad type: roomType,
    \State \quad position: position,
    \State \quad width: size.width,
    \State \quad height: size.height,
    \State \quad exits: []
    \State \}

    \State \Comment{Mark grid cells as occupied}
    \ForAll{x $\in [position.x, position.x + size.width)$}
        \ForAll{z $\in [position.z, position.z + size.height)$}
            \State grid[x][z] $\gets$ room.id
        \EndFor
    \EndFor

    \State \Return room
\EndFunction

\end{algorithmic}
\end{algorithm}

\subsection{Unique Feature Generation}

The system adds unique architectural and magical features based on castle type and randomness factors.

\begin{algorithm}[!htbp]
\caption{Unique Feature Generation and Placement}
\label{alg:unique-features}
\begin{algorithmic}[1]
\Require Castle type, Configuration, Uniqueness factor $u \in [0, 1]$
\Ensure Placed unique features

\Function{GenerateUniqueFeatures}{castleType, config}
    \State features $\gets []$
    \State uniqueness $\gets$ config.uniqueness

    \State \Comment{Base features by castle type}
    \If{castleType = 'mystical'}
        \State \Call{Add}{features, 'floating\_crystals'}
        \State \Call{Add}{features, 'magical\_aura'}
    \ElsIf{castleType = 'fortress'}
        \State \Call{Add}{features, 'siege\_weapons'}
        \State \Call{Add}{features, 'reinforced\_gates'}
    \ElsIf{castleType = 'dark'}
        \State \Call{Add}{features, 'gargoyles'}
        \State \Call{Add}{features, 'shadow\_portals'}
    \EndIf

    \State \Comment{Rare features based on uniqueness}
    \If{uniqueness $> 0.8$}
        \State \Call{Add}{features, 'ancient\_runes'}
        \If{\Call{Random}{} $< 0.3$}
            \State \Call{Add}{features, 'hidden\_treasure'}
        \EndIf
    \EndIf

    \If{uniqueness $> 0.9$}
        \State \Call{Add}{features, 'legendary\_artifact'}
        \State \Call{Add}{features, 'guardian\_spirit'}
    \EndIf

    \If{uniqueness $> 0.95$ \textbf{and} castleType = 'mystical'}
        \State \Call{Add}{features, 'dimensional\_rift'}
    \EndIf

    \State \Return features
\EndFunction

\Function{PlaceFeature}{feature, structure}
    \State placement $\gets$ \Call{GetFeaturePlacement}{feature}

    \If{feature = 'floating\_crystals'}
        \State count $\gets$ \Call{RandomInt}{3, 8}
        \ForAll{i $\in [0, count)$}
            \State crystal $\gets$ \Call{CreateCrystal}{}
            \State position $\gets$ \Call{RandomPosition}{structure.bounds}
            \State position.y $\gets$ position.y $+ 10 + \Call{Random}{} \times 5$
            \State crystal.position $\gets$ position
            \State \Call{AddFloatingAnimation}{crystal}
            \State \Call{AttachTo}{structure, crystal}
        \EndFor

    \ElsIf{feature = 'ancient\_runes'}
        \State runePositions $\gets$ \Call{CalculateRuneCircle}{structure.center, 5}
        \ForAll{position $\in$ runePositions}
            \State rune $\gets$ \Call{CreateRune}{\Call{RandomInt}{1, 12}}
            \State rune.position $\gets$ position
            \State \Call{AddGlowEffect}{rune}
            \State \Call{AttachTo}{structure, rune}
        \EndFor

    \ElsIf{feature = 'hidden\_treasure'}
        \State treasureRoom $\gets$ \Call{SelectSecretLocation}{structure}
        \State treasure $\gets$ \Call{GenerateTreasure}{}
        \State \Call{PlaceInRoom}{treasureRoom, treasure}
        \State \Call{AddPuzzleDoor}{treasureRoom}

    \ElsIf{feature = 'guardian\_spirit'}
        \State spirit $\gets$ \Call{CreateGuardianSpirit}{structure.style}
        \State spirit.patrolPath $\gets$ \Call{GeneratePatrolPath}{structure}
        \State spirit.dormant $\gets$ true
        \State \Call{AttachTo}{structure, spirit}
    \EndIf
\EndFunction

\Function{GenerateCastleLore}{castleType, biome}
    \State loreDatabase $\gets$ \{
    \State \quad classic: \{
    \State \quad \quad temperate: "Noble stronghold of ancient kings",
    \State \quad \quad desert: "Fortress carved from sandstone cliffs",
    \State \quad \quad arctic: "Frozen bastion of the north",
    \State \quad \quad forest: "Keep hidden within ancient woods",
    \State \quad \quad volcanic: "Citadel forged in dragon fire"
    \State \quad \},
    \State \quad mystical: \{
    \State \quad \quad temperate: "Tower of arcane knowledge",
    \State \quad \quad forest: "Elven spire of living wood",
    \State \quad \quad volcanic: "Sanctum of elemental magic",
    \State \quad \quad arctic: "Crystal palace of ice magic",
    \State \quad \quad desert: "Mirage fortress of sand sorcery"
    \State \quad \},
    \State \quad dark: \{
    \State \quad \quad temperate: "Cursed castle of fallen nobility",
    \State \quad \quad forest: "Shadow keep of the dark woods",
    \State \quad \quad volcanic: "Demon fortress of the underworld",
    \State \quad \quad arctic: "Frozen tomb of ancient evil",
    \State \quad \quad desert: "Necropolis of the sand wraiths"
    \State \quad \}
    \State \}

    \State baseLore $\gets$ loreDatabase[castleType][biome]

    \State \Comment{Add dynamic lore elements}
    \State age $\gets$ \Call{RandomInt}{100, 3000}
    \State builder $\gets$ \Call{GenerateBuilderName}{castleType}
    \State event $\gets$ \Call{GenerateHistoricEvent}{biome}

    \State lore $\gets$ baseLore + ". Built " + age + " years ago by " + builder
    \State lore $\gets$ lore + ". " + event

    \State \Return lore
\EndFunction

\end{algorithmic}
\end{algorithm}
