# Supplementary material for: Cognibit: From Digital Exhaustion to Real-World Connection Through Gamified Territory Control and LLM-Powered Twin Networking
Source: arXiv:2604.04351 source file (2026-12-01)
Supplement: Supplementary file 5 [file Q-performance-optimization.tex]

% Appendix Q - Performance Optimization Techniques
\section{Performance Optimization Techniques}

This appendix presents advanced performance optimization algorithms including a WASM-ready architecture with JavaScript fallback, memory pooling, and real-time profiling systems. Theoretical analysis (Appendix~U) predicts 10--50$\times$ speedups for computationally intensive operations when a compiled WebAssembly module is provided; the current implementation uses a JavaScript fallback path that maintains correctness while the WASM module is compiled separately.

\subsection{WebAssembly Batch Optimization}

The WASM-ready optimizer provides a framework for batch operations that can leverage native code execution when a compiled module is available, falling back to equivalent JavaScript otherwise.

\begin{algorithm}[!htbp]
\caption{WebAssembly Batch Optimization}
\label{alg:wasm-batch-optimization}
\begin{algorithmic}[1]
\Require Object list, Camera parameters, Screen dimensions
\Ensure Optimized visibility and LOD calculations

\State \textbf{Initialize:}
\State maxObjects $\gets 1000$ \Comment{Pre-allocated buffer size}
\State speedupFactor $\gets 10$ to $50$ \Comment{Expected performance gain}
\State wasmAvailable $\gets$ \Call{CheckWASMSupport}{}

\Function{InitializeWASMOptimizer}{}
    \If{wasmAvailable}
        \State module $\gets$ \Call{LoadWASMModule}{'optimizer.wasm'}

        \State \Comment{Allocate memory buffers in WASM heap}
        \State positionsBuffer $\gets$ \Call{AllocateWASM}{maxObjects $\times 3 \times 4$} \Comment{3 floats}
        \State sizesBuffer $\gets$ \Call{AllocateWASM}{maxObjects $\times 4$}
        \State distancesBuffer $\gets$ \Call{AllocateWASM}{maxObjects $\times 4$}
        \State screenSizesBuffer $\gets$ \Call{AllocateWASM}{maxObjects $\times 4$}
        \State visibilityBuffer $\gets$ \Call{AllocateWASM}{maxObjects $\times 4$}

        \State \Comment{Create typed array views for zero-copy access}
        \State positionsView $\gets$ \Call{CreateFloat32View}{positionsBuffer, maxObjects $\times 3$}
        \State sizesView $\gets$ \Call{CreateFloat32View}{sizesBuffer, maxObjects}
        \State distancesView $\gets$ \Call{CreateFloat32View}{distancesBuffer, maxObjects}
        \State screenSizesView $\gets$ \Call{CreateFloat32View}{screenSizesBuffer, maxObjects}
        \State visibilityView $\gets$ \Call{CreateInt32View}{visibilityBuffer, maxObjects}

        \State \Return \{module, buffers, views\}
    \Else
        \State \Return null \Comment{Fallback to JavaScript}
    \EndIf
\EndFunction

\Function{OptimizeBatch}{camera, objects, screenHeight, maxDistance}
    \State count $\gets$ \Call{Min}{\Call{Size}{objects}, maxObjects}

    \If{wasmAvailable}
        \State \Return \Call{OptimizeBatchWASM}{camera, objects, count, screenHeight, maxDistance}
    \Else
        \State \Return \Call{OptimizeBatchJS}{camera, objects, count, screenHeight, maxDistance}
    \EndIf
\EndFunction

\Function{OptimizeBatchWASM}{camera, objects, count, screenHeight, maxDistance}
    \State \Comment{Step 1: Copy data to WASM memory (vectorized)}
    \ForAll{i $\in [0, count)$}
        \State obj $\gets$ objects[i]
        \State positionsView[i $\times 3$] $\gets$ obj.position.x
        \State positionsView[i $\times 3 + 1$] $\gets$ obj.position.y
        \State positionsView[i $\times 3 + 2$] $\gets$ obj.position.z

        \If{obj.boundingBox $\neq$ null}
            \State size $\gets$ \Call{CalculateBoundingSize}{obj.boundingBox}
        \Else
            \State size $\gets$ obj.scale $\times 5$ \Comment{Estimate}
        \EndIf
        \State sizesView[i] $\gets$ size
    \EndFor

    \State \Comment{Step 2: Get camera parameters}
    \State camPos $\gets$ camera.position
    \State camDir $\gets$ \Call{GetWorldDirection}{camera}
    \State fovRadians $\gets$ camera.fov $\times \pi / 180$

    \State \Comment{Step 3: Execute WASM function (SIMD optimized)}
    \State \Call{WASMExecute}{'optimizeBatch',
    \State \quad camPos.x, camPos.y, camPos.z,
    \State \quad camDir.x, camDir.z,
    \State \quad positionsBuffer, sizesBuffer,
    \State \quad distancesBuffer, screenSizesBuffer, visibilityBuffer,
    \State \quad count, fovRadians, screenHeight, maxDistance
    \State }

    \State \Comment{Step 4: Read results from WASM memory}
    \State distances $\gets$ \Call{ArrayFrom}{distancesView[0:count]}
    \State screenSizes $\gets$ \Call{ArrayFrom}{screenSizesView[0:count]}
    \State visibility $\gets$ \Call{ArrayFrom}{visibilityView[0:count]}

    \State \Return \{distances, screenSizes, visibility\}
\EndFunction

\Function{OptimizeBatchJS}{camera, objects, count, screenHeight, maxDistance}
    \State \Comment{JavaScript fallback - slower but compatible}
    \State distances $\gets []$
    \State screenSizes $\gets []$
    \State visibility $\gets []$

    \State camDir $\gets$ \Call{GetWorldDirection}{camera}
    \State tanHalfFov $\gets$ \Call{Tan}{camera.fov $\times \pi / 360$}

    \ForAll{i $\in [0, count)$}
        \State obj $\gets$ objects[i]

        \State \Comment{Calculate distance}
        \State dx $\gets$ obj.position.x - camera.position.x
        \State dy $\gets$ obj.position.y - camera.position.y
        \State dz $\gets$ obj.position.z - camera.position.z
        \State distance $\gets$ \Call{Sqrt}{dx$^2$ + dy$^2$ + dz$^2$}

        \State \Comment{Calculate screen size}
        \State objectSize $\gets$ \Call{GetObjectSize}{obj}
        \State screenSize $\gets$ (objectSize / distance) $\times$ screenHeight / (2 $\times$ tanHalfFov)

        \State \Comment{Determine visibility}
        \State dotProduct $\gets$ (dx $\times$ camDir.x + dz $\times$ camDir.z) / distance
        \State visible $\gets$ distance $< maxDistance$ \textbf{and} dotProduct $> 0$

        \State \Call{Add}{distances, distance}
        \State \Call{Add}{screenSizes, screenSize}
        \State \Call{Add}{visibility, visible ? 1 : 0}
    \EndFor

    \State \Return \{distances, screenSizes, visibility\}
\EndFunction

\end{algorithmic}
\end{algorithm}

\subsection{Real-Time Performance Profiling}

The profiling system identifies performance bottlenecks by measuring execution time of code sections with minimal overhead.

\begin{algorithm}[!htbp]
\caption{Performance Profiling and Bottleneck Detection}
\label{alg:performance-profiling}
\begin{algorithmic}[1]
\Require Code sections to profile, Frame budget (16.67ms for 60 FPS)
\Ensure Performance report with bottleneck identification

\State \textbf{Initialize:}
\State measurements $\gets$ Map() \Comment{Section name $\rightarrow$ timing data}
\State frameCount $\gets 0$
\State maxFrames $\gets 600$ \Comment{10 seconds at 60 FPS}
\State targetFrameTime $\gets 16.67$ms \Comment{60 FPS target}

\Function{ProfileSection}{sectionName, codeBlock}
    \If{\textbf{not} profilingEnabled}
        \State \Return \Call{Execute}{codeBlock}
    \EndIf

    \State \Call{StartMeasurement}{sectionName}
    \State result $\gets$ \Call{Execute}{codeBlock}
    \State \Call{EndMeasurement}{sectionName}

    \State \Return result
\EndFunction

\Function{StartMeasurement}{sectionName}
    \If{\textbf{not} \Call{Has}{measurements, sectionName}}
        \State measurements[sectionName] $\gets$ \{
        \State \quad totalTime: 0,
        \State \quad calls: 0,
        \State \quad maxTime: 0,
        \State \quad minTime: $\infty$,
        \State \quad samples: []
        \State \}
    \EndIf

    \State measurements[sectionName].startTime $\gets$ \Call{PerformanceNow}{}
\EndFunction

\Function{EndMeasurement}{sectionName}
    \State data $\gets$ measurements[sectionName]
    \If{data.startTime = null}
        \State \Return
    \EndIf

    \State elapsed $\gets$ \Call{PerformanceNow}{} - data.startTime

    \State \Comment{Update statistics}
    \State data.totalTime $\gets$ data.totalTime + elapsed
    \State data.calls $\gets$ data.calls + 1
    \State data.maxTime $\gets$ \Call{Max}{data.maxTime, elapsed}
    \State data.minTime $\gets$ \Call{Min}{data.minTime, elapsed}

    \State \Comment{Keep recent samples for variance analysis}
    \State \Call{Add}{data.samples, elapsed}
    \If{\Call{Size}{data.samples} $> 100$}
        \State \Call{RemoveFirst}{data.samples}
    \EndIf

    \State data.startTime $\gets$ null
\EndFunction

\Function{EndFrame}{}
    \If{\textbf{not} profilingEnabled}
        \State \Return
    \EndIf

    \State frameCount $\gets$ frameCount + 1

    \If{frameCount $\geq$ maxFrames}
        \State profilingEnabled $\gets$ false
        \State \Call{GenerateReport}{}
    \EndIf
\EndFunction

\Function{GenerateReport}{}
    \State results $\gets []$

    \ForAll{(name, data) $\in$ measurements}
        \State avgTime $\gets$ data.totalTime / data.calls
        \State variance $\gets$ \Call{CalculateVariance}{data.samples}
        \State percentOfFrame $\gets$ (avgTime / targetFrameTime) $\times 100$

        \State \Call{Add}{results, \{
        \State \quad name: name,
        \State \quad avgTime: avgTime,
        \State \quad maxTime: data.maxTime,
        \State \quad minTime: data.minTime,
        \State \quad variance: variance,
        \State \quad percentOfFrame: percentOfFrame,
        \State \quad calls: data.calls,
        \State \quad severity: \Call{ClassifySeverity}{percentOfFrame}
        \State \}}
    \EndFor

    \State \Comment{Sort by average time descending}
    \State \Call{Sort}{results, by: avgTime, descending}

    \State \Return \Call{FormatReport}{results}
\EndFunction

\Function{ClassifySeverity}{percentOfFrame}
    \If{percentOfFrame $> 30$}
        \State \Return 'CRITICAL' \Comment{Red flag}
    \ElsIf{percentOfFrame $> 15$}
        \State \Return 'WARNING' \Comment{Yellow flag}
    \ElsIf{percentOfFrame $> 5$}
        \State \Return 'MINOR' \Comment{Green flag}
    \Else
        \State \Return 'OPTIMAL'
    \EndIf
\EndFunction

\end{algorithmic}
\end{algorithm}

\subsection{Memory Pool Management}

Object pooling eliminates garbage collection overhead by reusing allocated objects.

\begin{algorithm}[!htbp]
\caption{High-Performance Object Pooling}
\label{alg:object-pooling}
\begin{algorithmic}[1]
\Require Object type, Pool size, Growth strategy
\Ensure Zero-allocation object reuse

\State \textbf{Pool Configuration:}
\State initialSize $\gets 100$
\State maxSize $\gets 1000$
\State growthFactor $\gets 1.5$

\Function{InitializeObjectPool}{objectType, initialSize}
    \State pool $\gets$ \{
    \State \quad available: [],
    \State \quad inUse: Set(),
    \State \quad objectType: objectType,
    \State \quad totalCreated: 0,
    \State \quad peakUsage: 0
    \State \}

    \State \Comment{Pre-allocate initial objects}
    \ForAll{i $\in [0, initialSize)$}
        \State obj $\gets$ \Call{CreateObject}{objectType}
        \State obj.poolId $\gets$ i
        \State \Call{Add}{pool.available, obj}
        \State pool.totalCreated $\gets$ pool.totalCreated + 1
    \EndFor

    \State \Return pool
\EndFunction

\Function{AcquireObject}{pool}
    \If{\Call{Size}{pool.available} = 0}
        \State \Call{GrowPool}{pool}
    \EndIf

    \If{\Call{Size}{pool.available} = 0}
        \State \Return null \Comment{Pool exhausted}
    \EndIf

    \State obj $\gets$ \Call{Pop}{pool.available}
    \State \Call{Add}{pool.inUse, obj}

    \State \Comment{Reset object state}
    \State \Call{ResetObject}{obj}

    \State \Comment{Track peak usage}
    \State currentUsage $\gets$ \Call{Size}{pool.inUse}
    \State pool.peakUsage $\gets$ \Call{Max}{pool.peakUsage, currentUsage}

    \State \Return obj
\EndFunction

\Function{ReleaseObject}{pool, obj}
    \If{\textbf{not} \Call{Contains}{pool.inUse, obj}}
        \State \Return false \Comment{Object not from this pool}
    \EndIf

    \State \Call{Remove}{pool.inUse, obj}

    \State \Comment{Clear references to prevent memory leaks}
    \State \Call{ClearReferences}{obj}

    \State \Call{Add}{pool.available, obj}

    \State \Return true
\EndFunction

\Function{GrowPool}{pool}
    \If{pool.totalCreated $\geq$ maxSize}
        \State \Return false \Comment{Max size reached}
    \EndIf

    \State currentSize $\gets$ pool.totalCreated
    \State newSize $\gets$ \Call{Min}{
    \State \quad \Call{Floor}{currentSize $\times$ growthFactor},
    \State \quad maxSize
    \State }

    \State growthCount $\gets$ newSize - currentSize

    \ForAll{i $\in [0, growthCount)$}
        \State obj $\gets$ \Call{CreateObject}{pool.objectType}
        \State obj.poolId $\gets$ pool.totalCreated + i
        \State \Call{Add}{pool.available, obj}
    \EndFor

    \State pool.totalCreated $\gets$ newSize

    \State \Return true
\EndFunction

\Function{OptimizePool}{pool}
    \State \Comment{Shrink pool if underutilized}
    \State utilizationRate $\gets$ pool.peakUsage / pool.totalCreated

    \If{utilizationRate $< 0.3$ \textbf{and} pool.totalCreated $> initialSize$}
        \State targetSize $\gets$ \Call{Max}{
        \State \quad initialSize,
        \State \quad \Call{Floor}{pool.peakUsage $\times 1.5$}
        \State }

        \While{\Call{Size}{pool.available} $> 0$ \textbf{and} pool.totalCreated $> targetSize$}
            \State obj $\gets$ \Call{Pop}{pool.available}
            \State \Call{DestroyObject}{obj}
            \State pool.totalCreated $\gets$ pool.totalCreated - 1
        \EndWhile
    \EndIf

    \State \Comment{Reset peak usage for next optimization cycle}
    \State pool.peakUsage $\gets$ \Call{Size}{pool.inUse}
\EndFunction

\end{algorithmic}
\end{algorithm}

\subsection{Adaptive Quality Scaling}

Dynamic quality adjustment maintains target framerate by scaling visual fidelity based on performance metrics.

\begin{algorithm}[!htbp]
\caption{Adaptive Quality Scaling}
\label{alg:adaptive-quality}
\begin{algorithmic}[1]
\Require Target FPS, Quality levels, Performance metrics
\Ensure Stable framerate through dynamic quality adjustment

\State \textbf{Quality Levels:}
\State ULTRA, HIGH, MEDIUM, LOW, POTATO
\State \textbf{Target Metrics:}
\State targetFPS $\gets 60$
\State minFPS $\gets 30$
\State adaptationRate $\gets 0.1$

\Function{AdaptiveQualityController}{}
    \State qualityLevel $\gets$ MEDIUM
    \State fpsHistory $\gets []$
    \State historySize $\gets 60$ \Comment{1 second of frames}
    \State cooldown $\gets 0$
    \State cooldownDuration $\gets 120$ \Comment{2 seconds}
\EndFunction

\Function{UpdateQuality}{currentFPS}
    \State \Comment{Maintain FPS history}
    \State \Call{Add}{fpsHistory, currentFPS}
    \If{\Call{Size}{fpsHistory} $> historySize$}
        \State \Call{RemoveFirst}{fpsHistory}
    \EndIf

    \If{cooldown $> 0$}
        \State cooldown $\gets$ cooldown - 1
        \State \Return \Comment{Wait for stabilization}
    \EndIf

    \State avgFPS $\gets$ \Call{Average}{fpsHistory}
    \State variance $\gets$ \Call{Variance}{fpsHistory}

    \State \Comment{Determine adjustment direction}
    \If{avgFPS $< minFPS$}
        \State \Call{DecreaseQuality}{'emergency'}
    \ElsIf{avgFPS $< targetFPS \times 0.9$}
        \State \Call{DecreaseQuality}{'gradual'}
    \ElsIf{avgFPS $> targetFPS \times 1.1$ \textbf{and} variance $< 5$}
        \State \Call{IncreaseQuality}{'gradual'}
    \EndIf
\EndFunction

\Function{DecreaseQuality}{mode}
    \State qualitySettings $\gets$ \Call{GetQualitySettings}{qualityLevel}

    \If{mode = 'emergency'}
        \State \Comment{Aggressive reduction}
        \State qualitySettings.shadowResolution $\gets$ qualitySettings.shadowResolution / 2
        \State qualitySettings.textureResolution $\gets$ qualitySettings.textureResolution / 2
        \State qualitySettings.effectsEnabled $\gets$ false
        \State qualitySettings.postProcessing $\gets$ false
    \Else
        \State \Comment{Gradual reduction}
        \If{qualityLevel $> LOW$}
            \State qualityLevel $\gets$ qualityLevel - 1
        \EndIf
    \EndIf

    \State \Call{ApplyQualitySettings}{qualitySettings}
    \State cooldown $\gets$ cooldownDuration
\EndFunction

\Function{IncreaseQuality}{mode}
    \If{qualityLevel $< ULTRA$}
        \State qualityLevel $\gets$ qualityLevel + 1
        \State qualitySettings $\gets$ \Call{GetQualitySettings}{qualityLevel}
        \State \Call{ApplyQualitySettings}{qualitySettings}
        \State cooldown $\gets$ cooldownDuration
    \EndIf
\EndFunction

\Function{GetQualitySettings}{level}
    \State settings $\gets$ \{
    \State \quad ULTRA: \{
    \State \quad \quad shadowResolution: 4096,
    \State \quad \quad textureResolution: 2048,
    \State \quad \quad maxLOD: 0,
    \State \quad \quad effectsEnabled: true,
    \State \quad \quad postProcessing: true,
    \State \quad \quad particleCount: 1000,
    \State \quad \quad drawDistance: 500
    \State \quad \},
    \State \quad HIGH: \{
    \State \quad \quad shadowResolution: 2048,
    \State \quad \quad textureResolution: 1024,
    \State \quad \quad maxLOD: 1,
    \State \quad \quad effectsEnabled: true,
    \State \quad \quad postProcessing: true,
    \State \quad \quad particleCount: 500,
    \State \quad \quad drawDistance: 300
    \State \quad \},
    \State \quad MEDIUM: \{
    \State \quad \quad shadowResolution: 1024,
    \State \quad \quad textureResolution: 512,
    \State \quad \quad maxLOD: 2,
    \State \quad \quad effectsEnabled: true,
    \State \quad \quad postProcessing: false,
    \State \quad \quad particleCount: 250,
    \State \quad \quad drawDistance: 200
    \State \quad \},
    \State \quad LOW: \{
    \State \quad \quad shadowResolution: 512,
    \State \quad \quad textureResolution: 256,
    \State \quad \quad maxLOD: 3,
    \State \quad \quad effectsEnabled: false,
    \State \quad \quad postProcessing: false,
    \State \quad \quad particleCount: 100,
    \State \quad \quad drawDistance: 100
    \State \quad \},
    \State \quad POTATO: \{
    \State \quad \quad shadowResolution: 0, \Comment{Disabled}
    \State \quad \quad textureResolution: 128,
    \State \quad \quad maxLOD: 4,
    \State \quad \quad effectsEnabled: false,
    \State \quad \quad postProcessing: false,
    \State \quad \quad particleCount: 0,
    \State \quad \quad drawDistance: 50
    \State \quad \}
    \State \}

    \State \Return settings[level]
\EndFunction

\end{algorithmic}
\end{algorithm}
