# Supplementary material for: Cognibit: From Digital Exhaustion to Real-World Connection Through Gamified Territory Control and LLM-Powered Twin Networking
Source: arXiv:2604.04351 source file (2026-12-01)
Supplement: Supplementary file 6 [file R-team-territory.tex]

% Appendix R - Team-Based Territory Systems
\section{Team-Based Territory Systems}

This appendix details the team-based gameplay mechanics including faction assignment, city control, resource sharing, and cooperative territory management.

\subsection{Team Formation and Management}

The team system organizes players into factions with unique identities and strategic advantages.

\begin{algorithm}[!htbp]
\caption{Team Formation and Player Assignment}
\label{alg:team-formation}
\begin{algorithmic}[1]
\Require Player ID, Available teams, Balance constraints
\Ensure Balanced team assignment

\State \textbf{Team Definitions:}
\State teams $\gets$ \{
\State \quad air: \{name: 'Air Clan', color: 0x87CEEB, bonus: 'movement'\},
\State \quad water: \{name: 'Water Tribe', color: 0x4682B4, bonus: 'healing'\},
\State \quad fire: \{name: 'Fire Nation', color: 0xFF4500, bonus: 'damage'\},
\State \quad earth: \{name: 'Earth Kingdom', color: 0x8B4513, bonus: 'defense'\},
\State \quad lightning: \{name: 'Lightning Sect', color: 0xFFD700, bonus: 'speed'\},
\State \quad shadow: \{name: 'Shadow Guild', color: 0x4B0082, bonus: 'stealth'\}
\State \}

\State playerTeams $\gets$ Map() \Comment{playerId $\rightarrow$ teamId}
\State teamRoster $\gets$ Map() \Comment{teamId $\rightarrow$ player list}

\Function{AssignPlayerToTeam}{playerId, requestedTeam}
    \State \Comment{Check if player already assigned}
    \If{\Call{Has}{playerTeams, playerId}}
        \State oldTeam $\gets$ playerTeams[playerId]
        \State \Call{RemoveFromRoster}{teamRoster[oldTeam], playerId}
    \EndIf

    \State \Comment{Auto-balance if requested team is full}
    \If{requestedTeam = null \textbf{or} \Call{IsTeamFull}{requestedTeam}}
        \State requestedTeam $\gets$ \Call{SelectBalancedTeam}{}
    \EndIf

    \State \Comment{Assign player to team}
    \State playerTeams[playerId] $\gets$ requestedTeam
    \If{\textbf{not} \Call{Has}{teamRoster, requestedTeam}}
        \State teamRoster[requestedTeam] $\gets$ []
    \EndIf
    \State \Call{Add}{teamRoster[requestedTeam], playerId}

    \State \Comment{Apply team bonuses}
    \State \Call{ApplyTeamBonuses}{playerId, teams[requestedTeam].bonus}

    \State \Return requestedTeam
\EndFunction

\Function{SelectBalancedTeam}{}
    \State minSize $\gets \infty$
    \State candidateTeams $\gets []$

    \ForAll{teamId $\in$ \Call{Keys}{teams}}
        \State size $\gets$ \Call{Size}{teamRoster[teamId] || []}

        \If{size $< minSize$}
            \State minSize $\gets$ size
            \State candidateTeams $\gets$ [teamId]
        \ElsIf{size = minSize}
            \State \Call{Add}{candidateTeams, teamId}
        \EndIf
    \EndFor

    \State \Comment{Random selection from smallest teams}
    \State \Return \Call{RandomChoice}{candidateTeams}
\EndFunction

\Function{IsTeamFull}{teamId}
    \State maxTeamSize $\gets$ \Call{Ceiling}{totalPlayers / \Call{Size}{teams}}
    \State currentSize $\gets$ \Call{Size}{teamRoster[teamId] || []}
    \State \Return currentSize $\geq$ maxTeamSize $\times 1.2$ \Comment{20% tolerance}
\EndFunction

\end{algorithmic}
\end{algorithm}

\subsection{City Control Mechanics}

The city control system implements capture mechanics, ownership tracking, and territory-based resource generation.

\begin{algorithm}[!htbp]
\caption{City Control and Ownership Management}
\label{alg:city-control}
\begin{algorithmic}[1]
\Require City ID, Player ID, Team affiliation
\Ensure Updated city ownership and resource generation

\State \textbf{Initialize:}
\State cityControllers $\gets$ Map() \Comment{cityId $\rightarrow$ control info}
\State captureProgress $\gets$ Map() \Comment{cityId $\rightarrow$ capture state}
\State captureThreshold $\gets 100$ \Comment{Points needed to capture}
\State decayRate $\gets 0.5$ \Comment{Points/second when uncontested}

\Function{AttemptCityCapture}{cityId, playerId, deltaTime}
    \State playerTeam $\gets$ \Call{GetPlayerTeam}{playerId}
    \State currentController $\gets$ cityControllers[cityId]

    \State \Comment{Initialize capture progress if needed}
    \If{\textbf{not} \Call{Has}{captureProgress, cityId}}
        \State captureProgress[cityId] $\gets$ \{
        \State \quad progress: 0,
        \State \quad capturer: null,
        \State \quad team: null
        \State \}
    \EndIf

    \State capture $\gets$ captureProgress[cityId]

    \State \Comment{Check if city is contested}
    \State contestingPlayers $\gets$ \Call{GetPlayersInCity}{cityId}
    \State contestingTeams $\gets$ \Call{GetUniqueTeams}{contestingPlayers}

    \If{\Call{Size}{contestingTeams} $> 1$}
        \State \Return \Call{HandleContestedCapture}{cityId, contestingTeams}
    \EndIf

    \State \Comment{Single team capturing}
    \If{currentController = null \textbf{or} currentController.teamId $\neq$ playerTeam}
        \State \Call{UpdateCaptureProgress}{cityId, playerId, playerTeam, deltaTime}
    \Else
        \State \Call{ReinforceControl}{cityId, playerId, deltaTime}
    \EndIf
\EndFunction

\Function{UpdateCaptureProgress}{cityId, playerId, teamId, deltaTime}
    \State capture $\gets$ captureProgress[cityId]

    \State \Comment{Reset if different team starts capturing}
    \If{capture.team $\neq$ null \textbf{and} capture.team $\neq$ teamId}
        \State capture.progress $\gets 0$
        \State capture.team $\gets$ teamId
        \State capture.capturer $\gets$ playerId
    \EndIf

    \State \Comment{Increase capture progress}
    \State captureRate $\gets$ \Call{CalculateCaptureRate}{playerId, teamId}
    \State capture.progress $\gets$ capture.progress + captureRate $\times$ deltaTime

    \State \Comment{Check if capture complete}
    \If{capture.progress $\geq$ captureThreshold}
        \State \Call{CompleteCapture}{cityId, playerId, teamId}
        \State capture.progress $\gets 0$
    \EndIf

    \State \Comment{Update UI}
    \State \Call{UpdateCaptureUI}{cityId, capture.progress / captureThreshold}
\EndFunction

\Function{CompleteCapture}{cityId, playerId, teamId}
    \State previousController $\gets$ cityControllers[cityId]

    \State cityControllers[cityId] $\gets$ \{
    \State \quad playerId: playerId,
    \State \quad playerName: \Call{GetPlayerName}{playerId},
    \State \quad teamId: teamId,
    \State \quad teamName: teams[teamId].name,
    \State \quad controlledSince: \Call{Now}{},
    \State \quad defenseBonus: 1.0
    \State \}

    \State \Comment{Notify team members}
    \State teamMembers $\gets$ teamRoster[teamId]
    \ForAll{member $\in$ teamMembers}
        \State \Call{SendNotification}{member, "City captured!"}
    \EndFor

    \State \Comment{Transfer city resources to team}
    \If{previousController $\neq$ null}
        \State \Call{TransferCityResources}{previousController.teamId, teamId, cityId}
    \EndIf

    \State \Comment{Apply team-wide bonuses}
    \State \Call{UpdateTeamBonuses}{teamId}
\EndFunction

\Function{HandleContestedCapture}{cityId, contestingTeams}
    \State \Comment{Pause capture when multiple teams present}
    \State capture $\gets$ captureProgress[cityId]

    \If{capture.progress $> 0$}
        \State \Comment{Decay progress during contest}
        \State capture.progress $\gets$ \Call{Max}{0, capture.progress - decayRate}
        \State \Call{UpdateCaptureUI}{cityId, capture.progress / captureThreshold, 'contested'}
    \EndIf

    \State \Comment{Calculate team strengths}
    \State teamStrengths $\gets$ Map()
    \ForAll{team $\in$ contestingTeams}
        \State strength $\gets$ \Call{CalculateTeamStrength}{team, cityId}
        \State teamStrengths[team] $\gets$ strength
    \EndFor

    \State \Comment{Trigger combat if strength difference is small}
    \State maxStrength $\gets$ \Call{Max}{teamStrengths}
    \State minStrength $\gets$ \Call{Min}{teamStrengths}

    \If{maxStrength / minStrength $< 1.5$}
        \State \Call{TriggerTeamBattle}{cityId, contestingTeams}
    \EndIf
\EndFunction

\end{algorithmic}
\end{algorithm}

\subsection{Team Resource Sharing}

The resource sharing system enables cooperative gameplay through shared resources and team-wide benefits.

\begin{algorithm}[!htbp]
\caption{Team Resource Management and Sharing}
\label{alg:team-resources}
\begin{algorithmic}[1]
\Require Team ID, Resource types, Sharing policies
\Ensure Distributed resources and team benefits

\State \textbf{Resource Types:}
\State GOLD, EXPERIENCE, MATERIALS, TERRITORY\_POINTS

\State teamResources $\gets$ Map() \Comment{teamId $\rightarrow$ resource pools}
\State contributionTracking $\gets$ Map() \Comment{playerId $\rightarrow$ contributions}

\Function{InitializeTeamResources}{teamId}
    \State teamResources[teamId] $\gets$ \{
    \State \quad gold: 0,
    \State \quad experience: 0,
    \State \quad materials: 0,
    \State \quad territoryPoints: 0,
    \State \quad sharedInventory: [],
    \State \quad bonusMultiplier: 1.0
    \State \}
\EndFunction

\Function{ContributeResources}{playerId, teamId, resourceType, amount}
    \State resources $\gets$ teamResources[teamId]

    \State \Comment{Apply team bonus}
    \State effectiveAmount $\gets$ amount $\times$ resources.bonusMultiplier

    \State \Comment{Update team pool}
    \If{resourceType = GOLD}
        \State resources.gold $\gets$ resources.gold + effectiveAmount
    \ElsIf{resourceType = EXPERIENCE}
        \State resources.experience $\gets$ resources.experience + effectiveAmount
        \State \Call{DistributeExperience}{teamId, effectiveAmount}
    \ElsIf{resourceType = MATERIALS}
        \State resources.materials $\gets$ resources.materials + effectiveAmount
    \ElsIf{resourceType = TERRITORY\_POINTS}
        \State resources.territoryPoints $\gets$ resources.territoryPoints + effectiveAmount
    \EndIf

    \State \Comment{Track individual contributions}
    \If{\textbf{not} \Call{Has}{contributionTracking, playerId}}
        \State contributionTracking[playerId] $\gets$ \{total: 0, byType: Map()\}
    \EndIf

    \State contribution $\gets$ contributionTracking[playerId]
    \State contribution.total $\gets$ contribution.total + effectiveAmount
    \State contribution.byType[resourceType] $\gets$ (contribution.byType[resourceType] || 0) + effectiveAmount

    \State \Comment{Check for contribution milestones}
    \State \Call{CheckContributionMilestones}{playerId, contribution.total}
\EndFunction

\Function{DistributeExperience}{teamId, amount}
    \State members $\gets$ teamRoster[teamId]
    \State activeMembers $\gets$ \Call{GetActiveMembers}{members}

    \If{\Call{Size}{activeMembers} = 0}
        \State \Return
    \EndIf

    \State \Comment{Calculate distribution}
    \State baseShare $\gets$ amount $\times 0.7$ / \Call{Size}{activeMembers}
    \State bonusPool $\gets$ amount $\times 0.3$

    \ForAll{member $\in$ activeMembers}
        \State share $\gets$ baseShare

        \State \Comment{Add performance-based bonus}
        \State contribution $\gets$ contributionTracking[member].total || 0
        \State totalContribution $\gets$ \Call{Sum}{contributionTracking, 'total'}

        \If{totalContribution $> 0$}
            \State contributionRatio $\gets$ contribution / totalContribution
            \State share $\gets$ share + bonusPool $\times$ contributionRatio
        \EndIf

        \State \Call{GrantExperience}{member, share}
    \EndFor
\EndFunction

\Function{RequestTeamResource}{playerId, teamId, resourceType, amount}
    \State resources $\gets$ teamResources[teamId]

    \State \Comment{Check permission level}
    \State permission $\gets$ \Call{GetPlayerPermission}{playerId, teamId}

    \If{permission $< 'member'}
        \State \Return \{success: false, reason: 'insufficient\_permission'\}
    \EndIf

    \State \Comment{Check availability}
    \State available $\gets$ resources[resourceType] || 0

    \If{available $< amount$}
        \State \Return \{success: false, reason: 'insufficient\_resources'\}
    \EndIf

    \State \Comment{Apply withdrawal limits}
    \State dailyLimit $\gets$ \Call{GetDailyLimit}{playerId, resourceType}
    \State withdrawn $\gets$ \Call{GetDailyWithdrawn}{playerId, resourceType}

    \If{withdrawn + amount $> dailyLimit$}
        \State amount $\gets$ dailyLimit - withdrawn
    \EndIf

    \State \Comment{Transfer resources}
    \State resources[resourceType] $\gets$ resources[resourceType] - amount
    \State \Call{GrantResource}{playerId, resourceType, amount}

    \State \Comment{Log transaction}
    \State \Call{LogTransaction}{teamId, playerId, resourceType, -amount}

    \State \Return \{success: true, amount: amount\}
\EndFunction

\end{algorithmic}
\end{algorithm}

\subsection{Team Coordination Protocols}

Advanced coordination mechanics enable strategic team play through communication, objectives, and synchronized actions.

\begin{algorithm}[!htbp]
\caption{Team Coordination and Strategy System}
\label{alg:team-coordination}
\begin{algorithmic}[1]
\Require Team members, Objectives, Communication channels
\Ensure Coordinated team actions and strategic play

\State \textbf{Coordination States:}
\State IDLE, GATHERING, ATTACKING, DEFENDING, RAIDING

\State teamObjectives $\gets$ Map() \Comment{teamId $\rightarrow$ objective list}
\State teamStrategy $\gets$ Map() \Comment{teamId $\rightarrow$ current strategy}
\State rallyPoints $\gets$ Map() \Comment{teamId $\rightarrow$ location}

\Function{SetTeamObjective}{teamId, objectiveType, target, priority}
    \If{\textbf{not} \Call{Has}{teamObjectives, teamId}}
        \State teamObjectives[teamId] $\gets$ []
    \EndIf

    \State objective $\gets$ \{
    \State \quad id: \Call{GenerateId}{},
    \State \quad type: objectiveType,
    \State \quad target: target,
    \State \quad priority: priority,
    \State \quad createdAt: \Call{Now}{},
    \State \quad assignedMembers: [],
    \State \quad progress: 0,
    \State \quad status: 'active'
    \State \}

    \State \Call{Add}{teamObjectives[teamId], objective}

    \State \Comment{Auto-assign members based on priority}
    \If{priority = 'critical'}
        \State \Call{NotifyAllMembers}{teamId, objective}
        \State \Call{AutoAssignMembers}{teamId, objective}
    \EndIf

    \State \Return objective.id
\EndFunction

\Function{AutoAssignMembers}{teamId, objective}
    \State members $\gets$ teamRoster[teamId]
    \State availableMembers $\gets$ []

    \ForAll{member $\in$ members}
        \State currentTask $\gets$ \Call{GetCurrentTask}{member}

        \If{currentTask = null \textbf{or} currentTask.priority $< objective.priority$}
            \State \Call{Add}{availableMembers, member}
        \EndIf
    \EndFor

    \State \Comment{Assign based on objective type}
    \State requiredMembers $\gets$ \Call{CalculateRequiredMembers}{objective}
    \State assignedCount $\gets 0$

    \ForAll{member $\in$ availableMembers}
        \If{assignedCount $\geq$ requiredMembers}
            \State \textbf{break}
        \EndIf

        \State suitability $\gets$ \Call{CalculateSuitability}{member, objective}

        \If{suitability $> 0.5$}
            \State \Call{AssignToObjective}{member, objective}
            \State assignedCount $\gets$ assignedCount + 1
        \EndIf
    \EndFor
\EndFunction

\Function{CoordinateTeamAttack}{teamId, targetCity}
    \State \Comment{Set rally point}
    \State rallyLocation $\gets$ \Call{CalculateRallyPoint}{targetCity}
    \State rallyPoints[teamId] $\gets$ rallyLocation

    \State \Comment{Create attack objective}
    \State objective $\gets$ \Call{SetTeamObjective}{teamId, 'ATTACK', targetCity, 'critical'}

    \State \Comment{Coordinate timing}
    \State attackTime $\gets$ \Call{Now}{} + 60000 \Comment{1 minute preparation}
    \State members $\gets$ teamRoster[teamId]

    \ForAll{member $\in$ members}
        \State distance $\gets$ \Call{GetDistanceToTarget}{member, rallyLocation}
        \State travelTime $\gets$ distance / \Call{GetMovementSpeed}{member}
        \State departTime $\gets$ attackTime - travelTime

        \State \Call{ScheduleAction}{member, \{
        \State \quad action: 'move\_to\_rally',
        \State \quad location: rallyLocation,
        \State \quad time: departTime
        \State \}}

        \State \Call{ScheduleAction}{member, \{
        \State \quad action: 'attack\_city',
        \State \quad target: targetCity,
        \State \quad time: attackTime
        \State \}}
    \EndFor

    \State \Comment{Assign roles}
    \State \Call{AssignCombatRoles}{members, targetCity}

    \State \Return objective
\EndFunction

\Function{AssignCombatRoles}{members, target}
    \State roles $\gets$ \{
    \State \quad tanks: [],
    \State \quad damage: [],
    \State \quad support: [],
    \State \quad flankers: []
    \State \}

    \ForAll{member $\in$ members}
        \State stats $\gets$ \Call{GetPlayerStats}{member}

        \If{stats.defense $> 70$}
            \State \Call{Add}{roles.tanks, member}
        \ElsIf{stats.attack $> 70$}
            \State \Call{Add}{roles.damage, member}
        \ElsIf{stats.healing $> 50$}
            \State \Call{Add}{roles.support, member}
        \ElsIf{stats.speed $> 70$}
            \State \Call{Add}{roles.flankers, member}
        \Else
            \State \Comment{Assign to needed role}
            \State neededRole $\gets$ \Call{GetMostNeededRole}{roles}
            \State \Call{Add}{roles[neededRole], member}
        \EndIf
    \EndFor

    \State \Comment{Communicate roles to players}
    \ForAll{role, players $\in$ roles}
        \ForAll{player $\in$ players}
            \State \Call{SetCombatRole}{player, role}
            \State \Call{SendTacticalInfo}{player, role, target}
        \EndFor
    \EndFor
\EndFunction

\Function{CalculateTeamSynergy}{teamId}
    \State members $\gets$ teamRoster[teamId]
    \State synergy $\gets 1.0$

    \State \Comment{Class diversity bonus}
    \State uniqueClasses $\gets$ \Call{GetUniqueClasses}{members}
    \State classDiversity $\gets$ \Call{Size}{uniqueClasses} / \Call{Size}{members}
    \State synergy $\gets$ synergy + classDiversity $\times 0.2$

    \State \Comment{Activity synchronization bonus}
    \State activeMembers $\gets$ \Call{GetActiveMembers}{members}
    \State activityRate $\gets$ \Call{Size}{activeMembers} / \Call{Size}{members}
    \State synergy $\gets$ synergy + activityRate $\times 0.3$

    \State \Comment{Objective completion bonus}
    \State completedObjectives $\gets$ \Call{GetCompletedObjectives}{teamId, 3600000} \Comment{Last hour}
    \State synergy $\gets$ synergy + \Call{Min}{0.5, completedObjectives $\times 0.1$}

    \State \Comment{Territory control bonus}
    \State controlledCities $\gets$ \Call{GetControlledCities}{teamId}
    \State synergy $\gets$ synergy + \Call{Min}{0.3, \Call{Size}{controlledCities} $\times 0.05$}

    \State \Return synergy
\EndFunction

\end{algorithmic}
\end{algorithm}
