# Supplementary material for: Cognibit: From Digital Exhaustion to Real-World Connection Through Gamified Territory Control and LLM-Powered Twin Networking
Source: arXiv:2604.04351 source file (2026-12-01)
Supplement: Supplementary file 7 [file S-security-privacy.tex]

% Appendix S - Security and Privacy Implementation
\section{Security and Privacy Implementation}

This appendix details the comprehensive security measures implemented to protect user data, prevent attacks, and ensure privacy in the browser-based architecture.

\subsection{CSRF Protection Algorithm}

Cross-Site Request Forgery (CSRF) protection prevents unauthorized commands from being transmitted from a user that the web application trusts.

\begin{algorithm}[!htbp]
\caption{CSRF Token Generation and Validation}
\label{alg:csrf-protection}
\begin{algorithmic}[1]
\Require User session, Request method, Origin validation
\Ensure Protected state-changing operations

\State \textbf{Initialize:}
\State tokenLength $\gets 32$ bytes
\State headerName $\gets$ 'X-CSRF-Token'
\State sessionStorage $\gets$ BrowserStorage('session')
\State tokenLifetime $\gets 3600000$ \Comment{1 hour}

\Function{InitializeCSRFProtection}{}
    \State \Comment{Generate cryptographically secure token}
    \State token $\gets$ \Call{GenerateCSRFToken}{}

    \State \Comment{Store in session storage}
    \State \Call{Store}{sessionStorage, 'csrf\_token', token}
    \State \Call{Store}{sessionStorage, 'csrf\_timestamp', \Call{Now}{}}

    \State \Comment{Attach to all forms}
    \State \Call{AttachToForms}{token}

    \State \Comment{Intercept all HTTP requests}
    \State \Call{InterceptRequests}{token}

    \State \Return token
\EndFunction

\Function{GenerateCSRFToken}{}
    \State randomBytes $\gets$ \Call{CryptoRandom}{tokenLength}
    \State token $\gets$ ""

    \ForAll{byte $\in$ randomBytes}
        \State hex $\gets$ \Call{ToHex}{byte}
        \State token $\gets$ token + \Call{PadLeft}{hex, 2, '0'}
    \EndFor

    \State \Return token
\EndFunction

\Function{InterceptRequests}{token}
    \State \Comment{Override fetch API}
    \State originalFetch $\gets$ window.fetch

    \State window.fetch $\gets$ \textbf{function}(url, options) \{
        \If{options.method $\in$ ['POST', 'PUT', 'DELETE', 'PATCH']}
            \State \Comment{Add CSRF token to headers}
            \If{options.headers = null}
                \State options.headers $\gets$ \{\}
            \EndIf
            \State options.headers[headerName] $\gets$ token

            \State \Comment{Validate origin}
            \If{\textbf{not} \Call{ValidateOrigin}{url}}
                \State \textbf{throw} SecurityException("Invalid origin")
            \EndIf
        \EndIf

        \State \Return \Call{Execute}{originalFetch, url, options}
    \State \}
\EndFunction

\Function{ValidateCSRFToken}{requestToken}
    \State storedToken $\gets$ \Call{Retrieve}{sessionStorage, 'csrf\_token'}
    \State timestamp $\gets$ \Call{Retrieve}{sessionStorage, 'csrf\_timestamp'}

    \State \Comment{Check token match}
    \If{requestToken $\neq$ storedToken}
        \State \Return false
    \EndIf

    \State \Comment{Check token age}
    \If{\Call{Now}{} - timestamp $>$ tokenLifetime}
        \State \Return false
    \EndIf

    \State \Comment{Rotate token after validation}
    \If{\Call{ShouldRotate}{}}
        \State newToken $\gets$ \Call{GenerateCSRFToken}{}
        \State \Call{Store}{sessionStorage, 'csrf\_token', newToken}
        \State \Call{Store}{sessionStorage, 'csrf\_timestamp', \Call{Now}{}}
    \EndIf

    \State \Return true
\EndFunction

\end{algorithmic}
\end{algorithm}

\subsection{Rate Limiting with Sliding Window}

Rate limiting prevents abuse and ensures fair resource usage through a sliding window algorithm that tracks request frequency.

\begin{algorithm}[!htbp]
\caption{Sliding Window Rate Limiting}
\label{alg:rate-limiting}
\begin{algorithmic}[1]
\Require Request identifier, Time window, Maximum requests
\Ensure Throttled request rate within limits

\State \textbf{Configuration:}
\State windowSize $\gets 60000$ms \Comment{1 minute}
\State maxRequests $\gets 100$ \Comment{Per window}
\State maxLoginAttempts $\gets 5$
\State lockoutDuration $\gets 900000$ms \Comment{15 minutes}

\State requestHistory $\gets$ Map() \Comment{identifier $\rightarrow$ timestamps}
\State lockouts $\gets$ Map() \Comment{identifier $\rightarrow$ lockout time}

\Function{CheckRateLimit}{identifier, requestType}
    \State now $\gets$ \Call{CurrentTime}{}

    \State \Comment{Check if locked out}
    \If{\Call{Has}{lockouts, identifier}}
        \State lockoutEnd $\gets$ lockouts[identifier]
        \If{now $< lockoutEnd$}
            \State \Return \{allowed: false, reason: 'locked\_out'\}
        \Else
            \State \Call{Remove}{lockouts, identifier}
        \EndIf
    \EndIf

    \State \Comment{Get request history}
    \If{\textbf{not} \Call{Has}{requestHistory, identifier}}
        \State requestHistory[identifier] $\gets$ []
    \EndIf

    \State timestamps $\gets$ requestHistory[identifier]
    \State windowStart $\gets$ now - windowSize

    \State \Comment{Filter requests within window}
    \State recentRequests $\gets$ []
    \ForAll{timestamp $\in$ timestamps}
        \If{timestamp $> windowStart$}
            \State \Call{Add}{recentRequests, timestamp}
        \EndIf
    \EndFor

    \State \Comment{Determine limit based on request type}
    \State limit $\gets$ maxRequests
    \If{requestType = 'login'}
        \State limit $\gets$ maxLoginAttempts
    \EndIf

    \State \Comment{Check if limit exceeded}
    \If{\Call{Size}{recentRequests} $\geq$ limit}
        \If{requestType = 'login'}
            \State \Comment{Apply lockout for login failures}
            \State lockouts[identifier] $\gets$ now + lockoutDuration
        \EndIf
        \State \Return \{allowed: false, reason: 'rate\_limit\_exceeded'\}
    \EndIf

    \State \Comment{Add current request}
    \State \Call{Add}{recentRequests, now}
    \State requestHistory[identifier] $\gets$ recentRequests

    \State \Return \{allowed: true, remaining: limit - \Call{Size}{recentRequests}\}
\EndFunction

\Function{CreateAdaptiveRateLimiter}{baseLimit, adaptiveFactors}
    \State \Comment{Create limiter with dynamic adjustment}
    \State limiter $\gets$ \{
    \State \quad baseLimit: baseLimit,
    \State \quad currentLimit: baseLimit,
    \State \quad factors: adaptiveFactors,
    \State \quad history: []
    \State \}

    \State limiter.adjust $\gets$ \textbf{function}() \{
        \State \Comment{Adjust based on system load}
        \State cpuUsage $\gets$ \Call{GetCPUUsage}{}
        \State memoryUsage $\gets$ \Call{GetMemoryUsage}{}

        \If{cpuUsage $> 0.8$ \textbf{or} memoryUsage $> 0.8$}
            \State this.currentLimit $\gets$ this.baseLimit $\times 0.5$
        \ElsIf{cpuUsage $< 0.3$ \textbf{and} memoryUsage $< 0.3$}
            \State this.currentLimit $\gets$ this.baseLimit $\times 1.5$
        \Else
            \State this.currentLimit $\gets$ this.baseLimit
        \EndIf
    \State \}

    \State \Return limiter
\EndFunction

\Function{CleanupRateLimits}{}
    \State now $\gets$ \Call{CurrentTime}{}
    \State windowStart $\gets$ now - windowSize

    \ForAll{(identifier, timestamps) $\in$ requestHistory}
        \State validTimestamps $\gets$ []

        \ForAll{timestamp $\in$ timestamps}
            \If{timestamp $> windowStart$}
                \State \Call{Add}{validTimestamps, timestamp}
            \EndIf
        \EndFor

        \If{\Call{Size}{validTimestamps} = 0}
            \State \Call{Remove}{requestHistory, identifier}
        \Else
            \State requestHistory[identifier] $\gets$ validTimestamps
        \EndIf
    \EndFor
\EndFunction

\end{algorithmic}
\end{algorithm}

\subsection{Input Validation and Sanitization}

Comprehensive input validation prevents injection attacks and ensures data integrity through multi-layer validation.

\begin{algorithm}[!htbp]
\caption{Multi-Layer Input Validation Pipeline}
\label{alg:input-validation}
\begin{algorithmic}[1]
\Require User input, Validation rules, Sanitization policies
\Ensure Clean, validated, and safe input

\State \textbf{Validation Rules:}
\State maxInputLength $\gets 1000$
\State allowedFileTypes $\gets$ ['image/jpeg', 'image/png', 'image/webp']
\State maxFileSize $\gets 10 \times 1024 \times 1024$ \Comment{10MB}

\Function{ValidateAndSanitizeInput}{input, inputType, rules}
    \State \Comment{Step 1: Length validation}
    \If{\Call{Length}{input} $>$ maxInputLength}
        \State \Return \{valid: false, error: 'input\_too\_long'\}
    \EndIf

    \State \Comment{Step 2: Type-specific validation}
    \State validationResult $\gets$ \Call{ValidateByType}{input, inputType}
    \If{\textbf{not} validationResult.valid}
        \State \Return validationResult
    \EndIf

    \State \Comment{Step 3: Sanitization}
    \State sanitized $\gets$ \Call{SanitizeInput}{input, inputType}

    \State \Comment{Step 4: Content Security Check}
    \If{\Call{ContainsMaliciousPatterns}{sanitized}}
        \State \Return \{valid: false, error: 'malicious\_content'\}
    \EndIf

    \State \Comment{Step 5: Business rule validation}
    \If{rules $\neq$ null}
        \ForAll{rule $\in$ rules}
            \If{\textbf{not} \Call{ApplyRule}{sanitized, rule}}
                \State \Return \{valid: false, error: rule.errorMessage\}
            \EndIf
        \EndFor
    \EndIf

    \State \Return \{valid: true, value: sanitized\}
\EndFunction

\Function{ValidateByType}{input, type}
    \If{type = 'email'}
        \State pattern $\gets$ '^[^\\s@]+@[^\\s@]+\\.[^\\s@]+\$'
        \State \Return \{valid: \Call{Matches}{input, pattern}\}

    \ElsIf{type = 'username'}
        \State pattern $\gets$ '^[a-zA-Z0-9\_]\{3,20\}\$'
        \State \Return \{valid: \Call{Matches}{input, pattern}\}

    \ElsIf{type = 'password'}
        \State hasUpper $\gets$ \Call{Contains}{input, '[A-Z]'}
        \State hasLower $\gets$ \Call{Contains}{input, '[a-z]'}
        \State hasDigit $\gets$ \Call{Contains}{input, '[0-9]'}
        \State hasSpecial $\gets$ \Call{Contains}{input, '[!@\#\$\%\^{}\&*]'}
        \State isLongEnough $\gets$ \Call{Length}{input} $\geq 8$

        \State \Return \{valid: hasUpper \textbf{and} hasLower \textbf{and} hasDigit \textbf{and} hasSpecial \textbf{and} isLongEnough\}

    \ElsIf{type = 'url'}
        \State \Return \{valid: \Call{IsValidURL}{input}\}

    \ElsIf{type = 'file'}
        \State \Return \Call{ValidateFile}{input}

    \Else
        \State \Return \{valid: true\} \Comment{Default pass for unknown types}
    \EndIf
\EndFunction

\Function{SanitizeInput}{input, type}
    \State sanitized $\gets$ input

    \State \Comment{Remove null bytes}
    \State sanitized $\gets$ \Call{Replace}{sanitized, '\\x00', ''}

    \State \Comment{HTML entity encoding}
    \State htmlEntities $\gets$ \{
    \State \quad '<': '\&lt;',
    \State \quad '>': '\&gt;',
    \State \quad '"': '\&quot;',
    \State \quad "'": '\&\#x27;',
    \State \quad '/': '\&\#x2F;',
    \State \quad '\&': '\&amp;'
    \State \}

    \ForAll{(char, entity) $\in$ htmlEntities}
        \State sanitized $\gets$ \Call{ReplaceAll}{sanitized, char, entity}
    \EndFor

    \State \Comment{Type-specific sanitization}
    \If{type = 'sql'}
        \State sanitized $\gets$ \Call{EscapeSQL}{sanitized}
    \ElsIf{type = 'javascript'}
        \State sanitized $\gets$ \Call{EscapeJS}{sanitized}
    \ElsIf{type = 'filename'}
        \State sanitized $\gets$ \Call{SanitizeFilename}{sanitized}
    \EndIf

    \State \Return sanitized
\EndFunction

\Function{ContainsMaliciousPatterns}{input}
    \State maliciousPatterns $\gets$ [
    \State \quad '<script', 'javascript:', 'onerror=', 'onclick=',
    \State \quad 'DROP TABLE', 'DELETE FROM', '; --',
    \State \quad '../', '..\\textbackslash', '\%00', '\%0d\%0a',
    \State \quad 'eval(', 'setTimeout(', 'setInterval('
    \State ]

    \State lowerInput $\gets$ \Call{ToLower}{input}

    \ForAll{pattern $\in$ maliciousPatterns}
        \If{\Call{Contains}{lowerInput, pattern}}
            \State \Call{LogSecurityEvent}{'malicious\_pattern\_detected', pattern}
            \State \Return true
        \EndIf
    \EndFor

    \State \Return false
\EndFunction

\end{algorithmic}
\end{algorithm}

\subsection{Privacy-Preserving Location Obfuscation}

Location data is obfuscated to protect user privacy while maintaining functionality for location-based features.

\begin{algorithm}[!htbp]
\caption{Location Privacy Protection}
\label{alg:location-privacy}
\begin{algorithmic}[1]
\Require Precise location, Privacy level, Context
\Ensure Obfuscated location preserving privacy

\State \textbf{Privacy Levels:}
\State HIGH $\gets$ 1000m radius \Comment{City district level}
\State MEDIUM $\gets$ 500m radius \Comment{Neighborhood level}
\State LOW $\gets$ 100m radius \Comment{Street level}
\State MINIMAL $\gets$ 20m radius \Comment{Building level}

\Function{ObfuscateLocation}{location, privacyLevel, context}
    \State \Comment{Determine obfuscation radius}
    \State radius $\gets$ \Call{GetRadiusByLevel}{privacyLevel}

    \State \Comment{Add controlled random noise}
    \State angle $\gets$ \Call{Random}{} $\times 2\pi$
    \State distance $\gets$ \Call{Random}{} $\times$ radius

    \State \Comment{Calculate offset in meters}
    \State latOffset $\gets$ distance $\times$ \Call{Cos}{angle} / 111111
    \State lngOffset $\gets$ distance $\times$ \Call{Sin}{angle} / (111111 $\times$ \Call{Cos}{location.lat})

    \State obfuscated $\gets$ \{
    \State \quad lat: location.lat + latOffset,
    \State \quad lng: location.lng + lngOffset,
    \State \quad accuracy: radius,
    \State \quad timestamp: \Call{RoundToMinute}{\Call{Now}{}},
    \State \quad privacyLevel: privacyLevel
    \State \}

    \State \Comment{Apply k-anonymity}
    \If{context.requireKAnonymity}
        \State obfuscated $\gets$ \Call{ApplyKAnonymity}{obfuscated, context.k}
    \EndIf

    \State \Comment{Apply differential privacy}
    \If{context.requireDifferentialPrivacy}
        \State obfuscated $\gets$ \Call{ApplyDifferentialPrivacy}{obfuscated, context.epsilon}
    \EndIf

    \State \Return obfuscated
\EndFunction

\Function{ApplyKAnonymity}{location, k}
    \State \Comment{Ensure at least k users in same area}
    \State gridSize $\gets$ \Call{CalculateGridSize}{k}
    \State gridCell $\gets$ \Call{SnapToGrid}{location, gridSize}

    \State usersInCell $\gets$ \Call{CountUsersInCell}{gridCell}

    \While{usersInCell $< k$}
        \State \Comment{Expand grid until k users found}
        \State gridSize $\gets$ gridSize $\times 2$
        \State gridCell $\gets$ \Call{SnapToGrid}{location, gridSize}
        \State usersInCell $\gets$ \Call{CountUsersInCell}{gridCell}
    \EndWhile

    \State \Return gridCell.center
\EndFunction

\Function{ApplyDifferentialPrivacy}{location, epsilon}
    \State \Comment{Add Laplacian noise for differential privacy}
    \State sensitivity $\gets 1.0$ \Comment{Maximum change in output}
    \State scale $\gets$ sensitivity / epsilon

    \State latNoise $\gets$ \Call{LaplacianRandom}{0, scale}
    \State lngNoise $\gets$ \Call{LaplacianRandom}{0, scale}

    \State location.lat $\gets$ location.lat + latNoise / 111111
    \State location.lng $\gets$ location.lng + lngNoise / (111111 $\times$ \Call{Cos}{location.lat})

    \State \Return location
\EndFunction

\Function{TemporalCloaking}{location, minDelay, maxDelay}
    \State \Comment{Delay location updates randomly}
    \State delay $\gets$ \Call{RandomInt}{minDelay, maxDelay}

    \State \Call{ScheduleAfter}{delay, \textbf{function}() \{
        \State \Call{TransmitLocation}{location}
    \State \}}

    \State \Comment{Batch with other updates if possible}
    \State \Call{AddToBatch}{location}

    \If{\Call{BatchSize}{} $\geq$ minBatchSize}
        \State \Call{FlushBatch}{}
    \EndIf
\EndFunction

\end{algorithmic}
\end{algorithm}

\subsection{Secure Data Storage and Encryption}

Client-side encryption ensures sensitive data remains protected even if storage is compromised.

\begin{algorithm}[!htbp]
\caption{Client-Side Encryption for Storage}
\label{alg:secure-storage}
\begin{algorithmic}[1]
\Require Data to store, Encryption key, Storage type
\Ensure Encrypted storage with integrity verification

\State \textbf{Encryption Parameters:}
\State algorithm $\gets$ 'AES-GCM'
\State keyLength $\gets 256$ bits
\State ivLength $\gets 12$ bytes
\State tagLength $\gets 128$ bits

\Function{SecureStore}{key, data, storageType}
    \State \Comment{Generate initialization vector}
    \State iv $\gets$ \Call{CryptoRandom}{ivLength}

    \State \Comment{Derive encryption key from master key}
    \State derivedKey $\gets$ \Call{DeriveKey}{key, storageType}

    \State \Comment{Serialize data}
    \State serialized $\gets$ \Call{JSONStringify}{data}

    \State \Comment{Encrypt with AES-GCM}
    \State encrypted $\gets$ \Call{EncryptAESGCM}{derivedKey, iv, serialized}

    \State \Comment{Create storage object}
    \State storageObject $\gets$ \{
    \State \quad iv: \Call{Base64Encode}{iv},
    \State \quad data: \Call{Base64Encode}{encrypted.ciphertext},
    \State \quad tag: \Call{Base64Encode}{encrypted.tag},
    \State \quad timestamp: \Call{Now}{},
    \State \quad version: 1
    \State \}

    \State \Comment{Add integrity check}
    \State storageObject.hmac $\gets$ \Call{ComputeHMAC}{derivedKey, storageObject}

    \State \Comment{Store based on type}
    \If{storageType = 'local'}
        \State \Call{LocalStorageSet}{key, storageObject}
    \ElsIf{storageType = 'session'}
        \State \Call{SessionStorageSet}{key, storageObject}
    \ElsIf{storageType = 'indexed'}
        \State \Call{IndexedDBSet}{key, storageObject}
    \EndIf

    \State \Return true
\EndFunction

\Function{SecureRetrieve}{key, storageType}
    \State \Comment{Retrieve encrypted data}
    \State storageObject $\gets$ null

    \If{storageType = 'local'}
        \State storageObject $\gets$ \Call{LocalStorageGet}{key}
    \ElsIf{storageType = 'session'}
        \State storageObject $\gets$ \Call{SessionStorageGet}{key}
    \ElsIf{storageType = 'indexed'}
        \State storageObject $\gets$ \Call{IndexedDBGet}{key}
    \EndIf

    \If{storageObject = null}
        \State \Return null
    \EndIf

    \State \Comment{Verify integrity}
    \State expectedHMAC $\gets$ \Call{ComputeHMAC}{key, storageObject}
    \If{storageObject.hmac $\neq$ expectedHMAC}
        \State \Call{LogSecurityEvent}{'integrity\_check\_failed', key}
        \State \Return null
    \EndIf

    \State \Comment{Decrypt data}
    \State derivedKey $\gets$ \Call{DeriveKey}{key, storageType}
    \State iv $\gets$ \Call{Base64Decode}{storageObject.iv}
    \State ciphertext $\gets$ \Call{Base64Decode}{storageObject.data}
    \State tag $\gets$ \Call{Base64Decode}{storageObject.tag}

    \State decrypted $\gets$ \Call{DecryptAESGCM}{derivedKey, iv, ciphertext, tag}

    \If{decrypted = null}
        \State \Call{LogSecurityEvent}{'decryption\_failed', key}
        \State \Return null
    \EndIf

    \State \Comment{Parse and return data}
    \State data $\gets$ \Call{JSONParse}{decrypted}
    \State \Return data
\EndFunction

\Function{RotateEncryptionKeys}{}
    \State \Comment{Periodic key rotation}
    \State oldKey $\gets$ currentKey
    \State newKey $\gets$ \Call{GenerateKey}{keyLength}

    \State \Comment{Re-encrypt all data}
    \ForAll{storageType $\in$ ['local', 'session', 'indexed']}
        \State items $\gets$ \Call{GetAllItems}{storageType}

        \ForAll{item $\in$ items}
            \State data $\gets$ \Call{SecureRetrieve}{item.key, storageType, oldKey}
            \If{data $\neq$ null}
                \State \Call{SecureStore}{item.key, data, storageType, newKey}
            \EndIf
        \EndFor
    \EndFor

    \State currentKey $\gets$ newKey
    \State \Call{SecurelyDeleteKey}{oldKey}
\EndFunction

\end{algorithmic}
\end{algorithm}
