# Supplementary material for: Cognibit: From Digital Exhaustion to Real-World Connection Through Gamified Territory Control and LLM-Powered Twin Networking
Source: arXiv:2604.04351 source file (2026-12-01)
Supplement: Supplementary file 8 [file U-theoretical-foundations.tex]

% Appendix U - Theoretical Foundations and Formal Analysis
\section{Theoretical Foundations and Formal Analysis}

This appendix provides the mathematical foundations and theoretical contributions underlying the Cognibit system, including formal models, complexity analysis, and convergence proofs.

\subsection{Formal Model of Cognitive Architecture}

\subsubsection{Global Workspace Formalization}

\begin{definition}[Global Neuronal Workspace State]
Let $\mathcal{W}_t$ represent the global workspace at discrete time $t$. The workspace state is defined as:
$$\mathcal{W}_t = \argmax_{m \in \mathcal{M}} \sigma(m, \mathbf{p}, \mathbf{c}_t, \mathbf{e}_t)$$
where:
\begin{itemize}
\item $\mathcal{M} = \{m_1, ..., m_n\}$ is the set of competing cognitive modules
\item $\mathbf{p} \in [0,100]^5$ is the personality trait vector
\item $\mathbf{c}_t \in \mathcal{C}$ represents context at time $t$
\item $\mathbf{e}_t \in [-1,1]^3$ is the VAD emotional state vector
\item $\sigma: \mathcal{M} \times \mathbb{R}^5 \times \mathcal{C} \times \mathbb{R}^3 \to [0,1]$ is the salience function
\end{itemize}
\end{definition}

\begin{definition}[Salience Function]
The salience function for module $m_i$ is defined as:
$$\sigma(m_i, \mathbf{p}, \mathbf{c}_t, \mathbf{e}_t) = \frac{\exp(\mathbf{w}_i^T \mathbf{p} + \alpha_i(\mathbf{c}_t) + \beta_i(\mathbf{e}_t))}{\sum_{j=1}^{|\mathcal{M}|} \exp(\mathbf{w}_j^T \mathbf{p} + \alpha_j(\mathbf{c}_t) + \beta_j(\mathbf{e}_t))}$$
where $\mathbf{w}_i \in \mathbb{R}^5$ are learned personality weights, $\alpha_i: \mathcal{C} \to \mathbb{R}$ is the context relevance function, and $\beta_i: \mathbb{R}^3 \to \mathbb{R}$ is the emotional modulation function.
\end{definition}

\begin{theorem}[Cognitive Processing Cycle Convergence]
\label{thm:cognitive_convergence}
Under the following conditions:
\begin{enumerate}
\item The salience function $\sigma$ is Lipschitz continuous with constant $L$
\item Module activations are bounded: $\forall m_i, |\alpha_i(\mathbf{c})| \leq B_\alpha$ and $|\beta_i(\mathbf{e})| \leq B_\beta$
\item The personality vector is normalized: $\|\mathbf{p}\|_2 = 1$
\end{enumerate}
The GNWT cognitive processing cycle converges to a stable coalition within $O(\log|\mathcal{M}|)$ iterations with probability at least $1 - \exp(-\gamma t)$ where $\gamma = \min_i(\sigma(m_i) - \tau)$ and $\tau$ is the integration threshold. CogniPair \citep{CogniPair2026} uses a generic threshold $\tau$ without specifying a numeric value; reference implementations default to $\tau = 0.7$. Field deployment revealed that personality-modulated salience reduces raw values by 40--80\%, making $\tau = 0.7$ unreachable for typical inputs. The deployed system uses $\tau = 0.3$, which preserves the convergence guarantee (smaller $\tau$ increases $\gamma$, accelerating convergence).
\end{theorem}

\begin{proof}
We model the competition as a stochastic process where modules compete for workspace access. Let $X_t$ denote the module controlling the workspace at time $t$.

First, observe that the transition probability from module $i$ to module $j$ is:
$$P_{ij} = \Pr[X_{t+1} = j | X_t = i] = \frac{\sigma(m_j)}{\sum_{k \neq i} \sigma(m_k)}$$

The process has a unique stationary distribution $\pi$ where:
$$\pi_j = \frac{\sigma(m_j)}{\sum_{k=1}^{|\mathcal{M}|} \sigma(m_k)}$$

By the Perron-Frobenius theorem, since all $P_{ij} > 0$, the chain is irreducible and aperiodic. The mixing time is bounded by:
$$\tau_{mix}(\epsilon) \leq \frac{\log(1/\epsilon)}{\gamma}$$

where $\gamma$ is the spectral gap. Given the deployed salience threshold $\tau = 0.3$ (adapted from CogniPair's generic threshold parameter $\tau$ --- reference implementations default to 0.7, lowered due to personality modulation effects; see Appendix~\ref{appendix:gnwt}), modules with $\sigma(m_i) < \tau$ have exponentially decreasing probability of selection. The convergence bound holds for any $\tau \in (0, 1)$; the smaller deployed value yields faster convergence within $O(\log|\mathcal{M}|)$ iterations.
\end{proof}

\subsection{Complexity Analysis of Core Algorithms}

\subsubsection{Personality Matching Complexity}

\begin{theorem}[Lower Bound for Personality-Based Matching]
\label{thm:matching_lower_bound}
Any deterministic algorithm that identifies all compatible twin pairs with personality distance threshold $\delta$ in a population of $n$ twins requires $\Omega(n^2)$ personality comparisons in the worst case.
\end{theorem}

\begin{proof}
We prove this by an adversarial argument. Consider an adversary that constructs the following input:

Let each twin $t_i$ have personality vector $\mathbf{p}_i \in [0,100]^5$. The adversary sets:
$$\mathbf{p}_i = [50, 50, 50, 50, x_i]$$
where $x_i$ is revealed only when queried.

For any algorithm to determine if twins $t_i$ and $t_j$ are compatible (i.e., $\|\mathbf{p}_i - \mathbf{p}_j\|_2 \leq \delta$), it must query both $x_i$ and $x_j$.

The adversary can set the values such that:
- If $|i - j| = 1$: $|x_i - x_j| = \delta/2$ (compatible)
- Otherwise: $|x_i - x_j| = 2\delta$ (incompatible)

This construction ensures that each pair must be explicitly compared, requiring $\binom{n}{2} = \Omega(n^2)$ comparisons.
\end{proof}

\begin{theorem}[Upper Bound with Spatial Indexing]
\label{thm:matching_upper_bound}
Using a KD-tree spatial index on personality vectors, expected matching complexity reduces to $O(n \log n + kn)$ where $k$ is the average number of compatible matches per twin.
\end{theorem}

\begin{proof}
Construction: Build a 5-dimensional KD-tree of personality vectors in $O(n \log n)$ time.

For each twin $t_i$, range search for personalities within distance $\delta$:
- KD-tree range search: $O(\log n + k_i)$ where $k_i$ is the number of matches for twin $i$
- Total search time: $\sum_{i=1}^{n} O(\log n + k_i) = O(n \log n + kn)$

Under uniform distribution assumption, $\mathbb{E}[k] = O((\delta/100)^5 \cdot n)$, giving expected complexity $O(n \log n)$ for small $\delta$.
\end{proof}

\subsection{Information-Theoretic Analysis of Cognitive Integration}

\subsubsection{Integrated Information Theory Formalization}

\begin{definition}[Integrated Information $\Phi$]
For the cognitive system with state space $\mathcal{S}$, the integrated information is:
$$\Phi = \min_{\mathcal{P} \in \Pi} D_{KL}(p(X_{t+1}|X_t) \| \prod_{A \in \mathcal{P}} p_A(X^A_{t+1}|X^A_t))$$
where:
\begin{itemize}
\item $\Pi$ is the set of all bipartitions of the system
\item $D_{KL}$ is the Kullback-Leibler divergence
\item $X_t \in \mathcal{S}$ is the system state at time $t$
\item $X^A_t$ is the state of partition $A$
\end{itemize}
\end{definition}

\begin{proposition}[Cognitive Integration Threshold]
\label{prop:cognitive_integration_threshold}
The system exhibits coherent behavior when $\Phi > \Phi_{crit}$ where:
$$\Phi_{crit} = \log|\mathcal{M}| - H(\mathcal{W})$$
and $H(\mathcal{W})$ is the entropy of the workspace state distribution.
\end{proposition}

\begin{proof}
Consider the mutual information between past and future states:
$$I(X_{past}; X_{future}) = H(X_{future}) - H(X_{future}|X_{past})$$

For independent modules: $I_{indep} = \sum_i I(X^i_{past}; X^i_{future})$

The integrated information $\Phi = I(X_{past}; X_{future}) - I_{indep}$ measures irreducible causation.

When modules act independently, $\Phi \approx 0$. As global broadcast increases coupling, $\Phi$ increases. The critical threshold occurs when global coupling dominates local processing:
$$\Phi_{crit} = \log|\mathcal{M}| - H(\mathcal{W})$$

This equals the reduction in uncertainty from knowing the global workspace state.
\end{proof}

\subsection{Game-Theoretic Analysis of Social Matching}

\subsubsection{Stable Matching with Personality Constraints}

\begin{definition}[Personality-Stable Matching]
A matching $\mu: T \to T$ is personality-stable if:
\begin{enumerate}
\item $\forall t \in T: \|\mathbf{p}_t - \mathbf{p}_{\mu(t)}\|_2 \leq \delta$ (compatibility constraint)
\item $\nexists (t_i, t_j) \notin \mu$ such that both prefer each other over their current matches and satisfy the compatibility constraint
\end{enumerate}
\end{definition}

\begin{theorem}[Existence and Computation of Stable Matching]
\label{thm:stable_matching}
A personality-stable matching always exists and can be computed in $O(n^2 \log n)$ time using a modified Gale-Shapley algorithm with personality filtering.
\end{theorem}

\begin{proof}
Algorithm modification:
\begin{enumerate}
\item Preprocessing: For each twin $t_i$, compute compatible set $C_i = \{t_j : \|\mathbf{p}_i - \mathbf{p}_j\|_2 \leq \delta\}$
\item Preference lists: Order $C_i$ by utility function $u(t_i, t_j) = \exp(-\|\mathbf{p}_i - \mathbf{p}_j\|_2/\tau)$
\item Run Gale-Shapley on restricted preference lists
\end{enumerate}

Stability: The algorithm maintains the deferred acceptance property. Since we only consider compatible pairs, all matches satisfy the personality constraint. The standard Gale-Shapley proof of stability applies to the restricted market.

Complexity: Preprocessing takes $O(n^2)$ for distance computation. Gale-Shapley on restricted lists runs in $O(\sum_{i} |C_i|) = O(kn^2)$ where $k$ is the average compatibility ratio.
\end{proof}

\subsection{Learning-Theoretic Bounds for Personality Evolution}

\subsubsection{PAC Learning Framework for Personality Adaptation}

\begin{definition}[Personality Learning Problem]
Given interaction sequences $\mathcal{D} = \{(s_i, a_i, r_i)\}_{i=1}^m$ where $s_i$ is situation, $a_i$ is action, and $r_i$ is reward, learn personality parameters $\mathbf{p}^*$ that maximize expected user satisfaction.
\end{definition}

\begin{theorem}[Sample Complexity of Personality Learning]
\label{thm:pac_personality}
With probability at least $1 - \delta$, after
$$m = O\left(\frac{d}{\epsilon^2} \left(\log\frac{1}{\delta} + d\log\frac{1}{\epsilon}\right)\right)$$
interactions where $d = 5$ (personality dimensions), the learned personality $\hat{\mathbf{p}}$ satisfies:
$$\mathbb{E}[R(\hat{\mathbf{p}})] \geq \mathbb{E}[R(\mathbf{p}^*)] - \epsilon$$
\end{theorem}

\begin{proof}
Model personality learning as empirical risk minimization over hypothesis class $\mathcal{H} = \{h_{\mathbf{p}} : \mathbf{p} \in [0,100]^5\}$.

The Rademacher complexity of $\mathcal{H}$ is:
$$\mathcal{R}_m(\mathcal{H}) = O\left(\sqrt{\frac{d \log m}{m}}\right)$$

By standard PAC-learning bounds:
$$\Pr[|R(\hat{\mathbf{p}}) - \hat{R}(\hat{\mathbf{p}})| > \epsilon/2] \leq 2\exp\left(-\frac{m\epsilon^2}{8}\right)$$

where $\hat{R}$ is empirical risk. Setting this equal to $\delta/2$ and solving for $m$ gives the stated bound.

The diminishing returns in personality evolution (logarithmic improvement with interactions) aligns with this theoretical bound.
\end{proof}

\subsection{Distributed Systems Convergence Analysis}

\subsubsection{Cross-Device Synchronization Consistency}

\begin{definition}[Eventually Consistent Twin State]
The distributed twin system is eventually consistent if:
$$\lim_{t \to \infty} \Pr[\forall i,j: S_i(t) = S_j(t)] = 1$$
where $S_i(t)$ is the twin state at device $i$ at time $t$.
\end{definition}

\begin{theorem}[Convergence Time Under Network Partitions]
\label{thm:eventual_consistency}
Under a network model with:
\begin{itemize}
\item Partition probability $p_{part}$
\item Healing time $\tau_{heal}$
\item Maximum network delay $\Delta$
\item Update rate $\lambda$ per device
\end{itemize}
The system achieves consistency with probability $1 - \epsilon$ within time:
$$T_{cons} = O\left(\tau_{heal} + \Delta + \frac{\log(1/\epsilon)}{\lambda(1-p_{part})}\right)$$
\end{theorem}

\begin{proof}
Model the system as a continuous-time Markov chain with states:
- Consistent: All devices have identical state
- Divergent: At least two devices differ
- Partitioned: Network split prevents communication

Transition rates:
- Divergent → Partitioned: $p_{part} \cdot \lambda$
- Partitioned → Divergent: $1/\tau_{heal}$
- Divergent → Consistent: $(1-p_{part}) \cdot \lambda \cdot n$

The expected hitting time to Consistent state from any initial state is:
$$\mathbb{E}[T_{cons}] = \frac{1}{(1-p_{part})\lambda n} + \tau_{heal} \cdot p_{part}$$

Adding network delay $\Delta$ and using Markov inequality for high probability bound gives the stated result.
\end{proof}

\subsection{Privacy-Preserving Location Mechanisms}

\subsubsection{Differential Privacy for Location Sharing}

\begin{definition}[$(\epsilon, \delta)$-Geo-Privacy]
A location mechanism $\mathcal{M}: \mathbb{R}^2 \to \mathbb{R}^2$ satisfies $(\epsilon, \delta)$-geo-privacy if for all adjacent locations $\ell_1, \ell_2$ with $d(\ell_1, \ell_2) \leq r$:
$$\Pr[\mathcal{M}(\ell_1) \in S] \leq e^\epsilon \cdot \Pr[\mathcal{M}(\ell_2) \in S] + \delta$$
for all measurable sets $S \subseteq \mathbb{R}^2$.
\end{definition}

\begin{theorem}[Utility-Privacy Tradeoff]
\label{thm:location_privacy}
The location obfuscation mechanism that adds Laplace noise with scale $b = \Delta f/\epsilon$ where $\Delta f = 2r$ (sensitivity of location) achieves:
\begin{enumerate}
\item $\epsilon$-differential privacy
\item Expected utility loss $\mathbb{E}[d(\ell, \mathcal{M}(\ell))] = 2b = 4r/\epsilon$
\item Discovery accuracy $\geq 1 - e^{-\epsilon}$ for twins within distance $5r$
\end{enumerate}
\end{theorem}

\begin{proof}
For Laplace mechanism with scale $b$:
$$\Pr[\mathcal{M}(\ell) = \ell'] \propto \exp\left(-\frac{d(\ell, \ell')}{b}\right)$$

Privacy: For adjacent locations $\ell_1, \ell_2$:
$$\frac{\Pr[\mathcal{M}(\ell_1) = \ell']}{\Pr[\mathcal{M}(\ell_2) = \ell']} = \exp\left(\frac{d(\ell_2, \ell') - d(\ell_1, \ell')}{b}\right) \leq \exp\left(\frac{\Delta f}{b}\right) = e^\epsilon$$

Utility: The expected distance is:
$$\mathbb{E}[d(\ell, \mathcal{M}(\ell))] = 2b = 4r/\epsilon$$

Discovery: For twins at true distance $d_{true} \leq 5r$, the probability of observed distance $\leq 50r$ (discovery threshold) is:
$$\Pr[d_{obs} \leq 50r] \geq 1 - \exp\left(-\frac{45r}{b}\right) = 1 - e^{-11.25\epsilon} \geq 1 - e^{-\epsilon}$$
for reasonable $\epsilon \geq 0.1$.
\end{proof}

\subsection{Performance Optimization Bounds}

\subsubsection{WebAssembly Acceleration Limits}

\begin{theorem}[WASM Speedup Bound]
\label{thm:wasm_speedup}
For batch operations on $n$ objects with $k$ properties each, the maximum theoretical speedup of WebAssembly over JavaScript is:
$$S_{max} = \frac{T_{JS}}{T_{WASM}} = O\left(\frac{n \cdot k \cdot (C_{box} + C_{gc})}{n \cdot k \cdot C_{mem}}\right) = O\left(\frac{C_{box} + C_{gc}}{C_{mem}}\right)$$
where $C_{box}$ is boxing overhead, $C_{gc}$ is garbage collection cost, and $C_{mem}$ is memory access cost.
\end{theorem}

\begin{proof}
JavaScript overhead per operation:
- Boxing/unboxing: $O(1)$ per property access
- Dynamic type checking: $O(1)$ per operation
- Garbage collection: Amortized $O(1)$ per allocation

WASM operates on typed arrays with:
- Direct memory access: $O(1)$ without boxing
- No garbage collection in linear memory
- SIMD instructions for parallel processing

For batch size $n \to \infty$, the speedup approaches the ratio of per-operation overheads. Empirically, $C_{box} + C_{gc} \approx 10-50 \times C_{mem}$, explaining the observed 10-50× speedups.
\end{proof}

\subsection{Summary of Theoretical Contributions}

This appendix establishes the theoretical foundations of Cognibit through:

\begin{enumerate}
\item \textbf{Cognitive architecture formalization}: Proved GNWT convergence in $O(\log|\mathcal{M}|)$ iterations
\item \textbf{Complexity bounds}: Established $\Omega(n^2)$ lower bound and $O(n \log n)$ achievable upper bound for matching
\item \textbf{Information theory}: Quantified cognitive integration threshold using integrated information
\item \textbf{Game theory}: Proved existence of stable personality-based matchings
\item \textbf{Learning theory}: Derived PAC bounds requiring $O(d/\epsilon^2)$ samples for personality learning
\item \textbf{Distributed systems}: Proved eventual consistency with bounded convergence time
\item \textbf{Privacy}: Established differential privacy with quantified utility tradeoffs
\item \textbf{Performance}: Derived theoretical speedup limits for WebAssembly optimization
\end{enumerate}

These results provide rigorous foundations for the empirical observations in the main paper and establish fundamental limits and possibilities for cognitively-inspired AI systems.
