# Supplementary material for: Cognibit: From Digital Exhaustion to Real-World Connection Through Gamified Territory Control and LLM-Powered Twin Networking
Source: arXiv:2604.04351 source file (2026-12-01)
Supplement: Supplementary file 10 [file Y-reproducibility-guide.tex]

% Appendix Y - Reproducibility Guide
\section{Reproducibility Guide and Resources}

This appendix provides comprehensive instructions and resources for reproducing all experiments, ensuring scientific transparency and enabling future research.

\subsection{Code and Data Availability}

\subsubsection{Open Source Repository}
\begin{itemize}
\item \textbf{GitHub}: Available at \url{https://github.com/pairXbt/cognibit} for review
\item \textbf{License}: MIT License
\item \textbf{DOI}: Will be assigned upon acceptance
\item \textbf{Commit}: \texttt{main} branch as of submission date
\item \textbf{Size}: 487 MB (including assets) - WARNING: Large repository
\item \textbf{Languages}: JavaScript (72\%), HTML (15\%), CSS (8\%), Python (5\%)
\item \textbf{Note}: Due to high maintenance burden and security vulnerabilities, code may not run without significant updates to dependencies
\end{itemize}

\subsubsection{Dataset Release}
\begin{itemize}
\item \textbf{OSF Project}: \url{https://osf.io/XXXXX}
\item \textbf{Contents}:
  \begin{itemize}
  \item Anonymized interaction logs (N=20, 2.3GB)
  \item Survey responses (pre/post/follow-up)
  \item Personality profiles (synthetic + evolved)
  \item Performance metrics (system logs)
  \item Qualitative interview transcripts
  \end{itemize}
\item \textbf{Format}: JSON, CSV, and Parquet files
\item \textbf{Documentation}: DataDictionary.pdf included
\end{itemize}

\subsubsection{Model Checkpoints}
\begin{itemize}
\item Fine-tuned personality models: HuggingFace Hub
\item Trained embeddings: \texttt{embeddings/personality-v1.pkl}
\item Configuration files: \texttt{configs/*.json}
\end{itemize}

\subsection{System Requirements}

\subsubsection{Minimum Hardware}
\begin{verbatim}
CPU:      2.0 GHz dual-core (Intel i5 or AMD equivalent)
RAM:      4 GB (8 GB recommended)
GPU:      WebGL 2.0 support (integrated graphics sufficient)
Storage:  2 GB free space
Network:  Broadband internet (>1 Mbps)
Display:  1280x720 resolution
\end{verbatim}

\subsubsection{Recommended Hardware}
\begin{verbatim}
CPU:      3.0 GHz quad-core
RAM:      16 GB
GPU:      Dedicated graphics (2GB VRAM)
Storage:  10 GB SSD
Network:  25+ Mbps
Display:  1920x1080 or higher
\end{verbatim}

\subsubsection{Software Dependencies}
\begin{verbatim}
# Browser requirements
Chrome 120+, Safari 17+, Firefox 121+, Edge 120+

# Development environment
Node.js:     v18.17.0 or higher
npm:         v9.6.7 or higher
Python:      3.9+ (for analysis scripts)
Git:         2.25+

# Cloud services (accounts required)
Firebase:    Realtime Database + Auth
OpenAI API:  GPT-4o and GPT-4o-mini access
Google Maps: Geocoding API (optional)
\end{verbatim}

\subsection{Installation Instructions}

\subsubsection{Local Development Setup}

\begin{verbatim}
# 1. Clone repository
git clone https://github.com/[masked]/cognibit.git
cd cognibit
git checkout v1.0-paper

# 2. Install dependencies
npm install

# 3. Configure environment
cp .env.example .env
# Edit .env with your API keys:
# OPENAI_API_KEY=sk-...
# FIREBASE_API_KEY=...
# FIREBASE_AUTH_DOMAIN=...
# FIREBASE_DATABASE_URL=...

# 4. Initialize Firebase
npm run firebase:init

# 5. Build assets
npm run build

# 6. Start development server
npm run dev
# Opens at http://localhost:3000
\end{verbatim}

\subsubsection{Docker Deployment}

\begin{verbatim}
# Using Docker Compose (recommended)
docker-compose up -d

# Manual Docker build
docker build -t cognibit:latest .
docker run -p 3000:3000 \
  -e OPENAI_API_KEY=$OPENAI_API_KEY \
  -e FIREBASE_CONFIG='{"apiKey":"..."}' \
  cognibit:latest
\end{verbatim}

\subsubsection{Production Deployment}

\begin{verbatim}
# 1. Build production bundle
npm run build:prod

# 2. Deploy to Firebase Hosting
npm run deploy

# 3. Or deploy to custom server
rsync -avz dist/ user@server:/var/www/cognibit/

# 4. Configure nginx (example)
server {
    listen 443 ssl http2;
    server_name cognibit.example.com;

    ssl_certificate /path/to/cert.pem;
    ssl_certificate_key /path/to/key.pem;

    root /var/www/cognibit;
    index index.html;

    location / {
        try_files $uri $uri/ /index.html;
    }

    location /api {
        proxy_pass http://localhost:3001;
    }
}
\end{verbatim}

\subsection{Reproducing Experiments}

\subsubsection{Experiment 1: User Engagement Study}

\begin{verbatim}
# Setup
cd experiments/user-engagement

# Configure participant groups
python setup_participants.py \
  --groups 4 \
  --size 40 \
  --randomize \
  --seed 42

# Run experiment protocol
npm run experiment:engagement \
  --duration "2 weeks" \
  --sessions 5 \
  --metrics "engagement,authenticity,connection"

# Collect data
python collect_data.py \
  --output data/engagement_raw.json

# Analyze results
python analysis/engagement_analysis.py \
  --input data/engagement_raw.json \
  --output results/engagement_stats.csv \
  --plots results/figures/
\end{verbatim}

\subsubsection{Experiment 2: Cognitive Architecture Validation}

\begin{verbatim}
# Configure cognitive architecture tracking
export TRACK_PHI=true
export PHI_SAMPLE_RATE=100  # ms
export PHI_LOG_PATH=./data/phi_measurements.jsonl

# Run cognitive processing cycles
node src/cognitive/measure_phi.js \
  --iterations 1000 \
  --modules 5 \
  --conditions "active,idle,random,none"

# Calculate integrated information
python analysis/calculate_phi.py \
  --input data/phi_measurements.jsonl \
  --method "IIT3.0" \
  --partitions "all_bipartitions" \
  --output results/phi_values.csv
\end{verbatim}

\subsubsection{Experiment 3: Ablation Studies}

\begin{verbatim}
# Automated ablation runner
python run_ablations.py \
  --config configs/ablation_config.yaml \
  --components "all" \
  --trials 50 \
  --parallel 4

# Config file example (ablation_config.yaml):
ablations:
  - name: "no_gnwt"
    disable: ["cognitive_cycle", "global_workspace"]
    metrics: ["engagement", "coherence", "phi"]

  - name: "no_memory"
    disable: ["memory_store", "memory_retrieval"]
    metrics: ["continuity", "recall_accuracy"]

  - name: "timing_50ms"
    modify:
      COGNITIVE_CYCLE_MS: 50
    metrics: ["convergence_time", "cpu_usage"]
\end{verbatim}

\subsection{Random Seeds and Determinism}

All randomness sources controlled for reproducibility:

\begin{verbatim}
// JavaScript random seed
const seedrandom = require('seedrandom');
const rng = seedrandom('cognibit-2024', { state: true });
Math.random = rng;

// Personality generation seed
const personalitySeeds = {
  initial: 'personality-42',
  evolution: 'evolution-1337',
  variation: 'variation-2024'
};

// Python analysis seed
import numpy as np
import random
import torch

def set_all_seeds(seed=42):
    np.random.seed(seed)
    random.seed(seed)
    torch.manual_seed(seed)
    if torch.cuda.is_available():
        torch.cuda.manual_seed_all(seed)

# R analysis seed
set.seed(42)
\end{verbatim}

\subsection{Hyperparameter Configurations}

Complete hyperparameter specifications:

\begin{verbatim}
{
  // Deployment configuration (adapted from CogniPair)
  "cognitive_architecture": {
    "cycle_time_ms": 100,
    "salience_threshold": 0.3,  // CogniPair specified τ=0.7;
                                // lowered because personality modulation
                                // reduces raw salience by 40-80%,
                                // making 0.7 unreachable in practice
    "workspace_capacity": 7,    // Miller's 7 (CogniPair: 7+/-2)
    "module_count": 5,
    "boost_factor": 1.2,
    "decay_rate": 0.95
  },

  "personality": {
    "dimensions": 5,
    "range": [0, 100],
    "evolution_rate": 0.01,
    "mutation_probability": 0.05,
    "convergence_threshold": 0.95
  },

  "memory": {
    "capacity": 100,
    "importance_threshold": 0.7, // memory consolidation (distinct from salience threshold)
    "decay_tau": 86400000,       // 24 hours
    "consolidation_interval": 3600000  // 1 hour
  },

  "llm": {
    "model_primary": "gpt-4o",
    "model_cost_optimized": "gpt-4o-mini",
    "temperature": 0.8,         // generation stage
    "intent_temperature": 0.3,  // intent analysis stage
    "max_tokens": 300,
    "top_p": 0.9,
    "frequency_penalty": 0.3,
    "presence_penalty": 0.5,
    "context_window": 10
  },

  "matching": {
    "compatibility_threshold": 0.2,
    "distance_weight": 0.3,
    "personality_weight": 0.7,
    "max_distance_miles": 50
  }
}
\end{verbatim}

\subsection{Troubleshooting Guide}

Common issues and solutions:

\begin{table}[h]
\centering
\small
\begin{tabular}{ll}
\toprule
\textbf{Issue} & \textbf{Solution} \\
\midrule
"Firebase permission denied" & Check authentication and database rules \\
"OpenAI rate limit" & Reduce parallel users or implement queuing \\
"WebGL context lost" & Reduce texture size or implement recovery \\
"Memory leak warning" & Clear caches, check disposal of Three.js objects \\
"Cognitive cycle timeout" & Increase timeout or reduce module count \\
"Personality drift" & Check evolution rate and boundary conditions \\
"LLM hallucinations" & Adjust temperature and add fact-checking \\
"Cross-origin errors" & Configure CORS headers properly \\
\bottomrule
\end{tabular}
\end{table}

\subsection{Validation Scripts}

Verify correct reproduction:

\begin{verbatim}
# Run validation suite
npm test

# Specific validation checks
npm run test:cognitive      # Verify cognitive architecture implementation
npm run test:personality    # Check personality evolution
npm run test:memory         # Validate memory operations
npm run test:integration    # End-to-end tests

# Performance benchmarks
npm run benchmark
# Expected results:
# - Cognitive processing cycle: 3-5ms
# - Memory retrieval: <1ms
# - LLM response: 2-3s
# - Frame rate: 55-60 FPS

# Statistical reproduction
python validate_stats.py \
  --original results/paper_results.csv \
  --reproduced results/my_results.csv \
  --tolerance 0.05
\end{verbatim}

\subsection{Computational Resource Estimates}

For full reproduction:

\begin{table}[h]
\centering
\begin{tabular}{lccc}
\toprule
\textbf{Experiment} & \textbf{Compute Hours} & \textbf{Storage} & \textbf{API Cost} \\
\midrule
User study (N=20) & 180 & 15 GB & $\sim$\$250\textsuperscript{*} \\
Ablations (all) & 240 & 8 GB & \$180 \\
Human baseline & 40 & 3 GB & \$0 \\
Longitudinal & 520 & 25 GB & \$890 \\
Cross-cultural & 120 & 10 GB & \$350 \\
\midrule
\textbf{Total} & 1,100 & 61 GB & \$1,670 \\
\bottomrule
\end{tabular}
\caption{Resource requirements for complete reproduction. \textsuperscript{*}Actual deployment: \$246.24.}
\end{table}

\subsection{Contact and Support}

For reproduction assistance:
\begin{itemize}
\item \textbf{GitHub Issues}: Technical problems and bugs
\item \textbf{Email}: [masked]@university.edu (corresponding author)
\item \textbf{Discord}: [invite-link] for community support
\item \textbf{Office Hours}: Fridays 2-4pm EST (Zoom link on website)
\end{itemize}

\subsection{Version History}

\begin{verbatim}
v1.0.0 (2024-01-15): Initial paper release
v1.0.1 (2024-01-20): Fixed memory leak in cognitive processing cycle
v1.0.2 (2024-01-25): Added missing configuration files
v1.1.0 (2024-02-01): Cross-cultural extensions
v1.2.0 (2024-02-15): Performance optimizations
\end{verbatim}

\subsection{Reproducibility Checklist}

\begin{itemize}
\item [$\square$] Code downloaded and builds successfully
\item [$\square$] Environment variables configured
\item [$\square$] Firebase project created and initialized
\item [$\square$] OpenAI API key obtained and tested
\item [$\square$] Sample experiment runs without errors
\item [$\square$] Validation tests pass
\item [$\square$] Performance benchmarks within 20\% of reported
\item [$\square$] Statistical results reproduce within tolerance
\item [$\square$] Ablation results consistent with paper
\item [$\square$] Can generate new twins with personalities
\end{itemize}

\subsection{Known Limitations}

Current reproduction limitations:
\begin{itemize}
\item GPT-4o model versions may differ (use gpt-4o-2024-05-13 for consistency)
\item Browser WebGL implementations vary slightly
\item Firebase free tier limits concurrent users to 100
\item Some randomness from user interactions cannot be controlled
\item Cross-cultural results may vary with participant populations
\end{itemize}

This comprehensive guide should enable complete reproduction of our results. We encourage researchers to report successful reproductions and any discrepancies to improve scientific transparency.
